# Supplementary material for: Nonlinear fractional waves at elastic interfaces
Source: arXiv:1702.08864 ancillary file (2017-02-28)
Supplement: Supplementary file 1 [file Supplement.pdf]

# Nonlinear fractional waves at elastic interfaces - Supplemental Information

Julian Kappler,[1] Shamit Shrivastava,[2] Matthias F. Schneider,[3] and Roland R. Netz[1]
[1]*Department of Physics, Freie Universität Berlin, Germany*
[2]*Institute of Biomedical Engineering, University of Oxford, United Kingdom*
[3]*Department of Physics, TU Dortmund, Germany*
(Dated: February 28, 2017)

In this supplement, we present detailed derivations, the numerical algorithm we use, and show the robustness of our nonlinear theory with respect to varying both elastic modulus and boundary condition.

In sect. S I, we start by reviewing the derivation of the Lucassen dispersion relation, and show that the displacement is mainly parallel to the interface. Then, in sect. S II, we provide an alternative derivation of the fractional wave equation, directly from momentum conservation and the stress boundary conditions at the interface.

After having established the linear fractional wave equation, we discuss the elastic modulus $K_{2D}$ in more detail: In sect. S III, we explain how we obtain $K_{2D}$ from an experimentally measured Langmuir isotherm, and in sect. S V discuss the assumption that the elastic modulus relevant for the Lucassen wave is isothermal. We finish our discussion of the elastic modulus in sect. S IV, where we discuss the assumption that nonlinear effects due to local changes in the elastic modulus $K_{2D}$ become relevant at smaller wave amplitudes than the convective nonlinear term in the momentum conservation equation.

In sect. S VI, we review the well-known analytical solution of the linear fractional wave equation. In the following sect. S VII, we explain the algorithm we use for numerically solving the nonlinear fractional wave equation. In sect. S VIII, we validate this numerical algorithm by comparing results of numerical solutions of the linear fractional wave equation to the corresponding analytical solutions.

In sect. S IX, we explain how we obtain a boundary condition for our numerical calculations from experimental data. Finally, in sect. S X we show that the numerical results presented in the main text are robust with respect to varying both the elastic modulus and the boundary condition.

## CONTENTS

S I. Standard derivation of Lucassen's dispersion relation 2
A. Linearized Navier-Stokes equation 2
B. Stress boundary conditions for a viscoelastic interface 2
C. Harmonic wave ansatz and implicit dispersion relation 4
D. Factorization of the implicit dispersion relation and Lucassen dispersion relation 5
E. Discussion of the factorization conditions for Lucassen waves in a lipid monolayer on water 5
F. Identification of the dominating term in the displacement field of the Lucassen wave 6

S II. Direct derivation of the fractional wave equation from momentum conservation and stress boundary conditions 7

S III. Numerical details for the calculation of the elastic modulus $K_{2D}$ 9

S IV. Discussion of the linearization assumption for momentum conservation 9

S V. Isothermal vs. adiabatic elastic modulus 10

S VI. Analytical solution of linear theory 11

S VII. Numerical algorithm for solving the nonlinear fractional wave equation 12
A. Introduction 12
B. Methods 13
C. Special case: Linear theory 14

S VIII. Linear theory: Comparison of analytical and numerical results 15
A. Introduction 15
B. Parameters 15
C. Position and time dependence of solutions at fixed $K_{2D}$ 15
D. Elastic modulus depedence of compression and wave velocity at fixed position $x$ 17
E. Conclusion 17

S IX. Obtaining the numerical boundary condition from experimental data 18

S X. Robustness of nonlinear numerical results with respect to varying elastic modulus and boundary condition 18
A. Varying the elastic modulus 19
B. Different boundary conditions 19

References 20

## S I. STANDARD DERIVATION OF LUCASSEN'S DISPERSION RELATION

In this section, we give a short derivation of the Lucassen dispersion relation. Most of this section is a summary of the calculations given in ref. [1]. Throughout this SI, we use Cartesian coordinates $\vec{r} = (x, y, z)$.

We consider a viscous incompressible fluid in the lower half space, $z \leq 0$ of $\mathbb{R}^3$, bounded by a viscoelastic interface at $z = 0$. Gravitational acceleration acts in the negative $z$-direction and couples to both the half space and the interface, c.f. fig. S1.

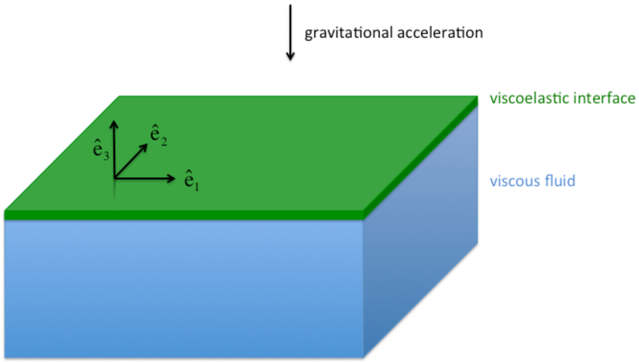


FIG. S1. **Setup.** We consider an incompressible viscous fluid with mass density $\rho$ and shear viscosity $\eta$ in the lower half space $z \leq 0$, bounded by a viscoelastic interface at $z = 0$ with area mass density $\rho_{2\mathrm{D}}$ and elastic modulus $K_{2\mathrm{D}}$. Gravitational acceleration $g$ points in the negative $z$-direction and couples to both the fluid and the interface.

### A. Linearized Navier-Stokes equation

For the bulk medium at $z < 0$, the linearized Navier-Stokes equation is given as [2]

$$\rho\, \partial_t v_i(\vec{r}, t) = \partial_j \sigma_{ij} + F_i(\vec{r}, t) \qquad i \in \{x, y, z\}, \tag{S1}$$

where $\vec{v}(\vec{r}, t)$ is the velocity field, $\vec{F}(\vec{r}, t)$ an external force, $\rho$ is the mass density, which is assumed to be constant, $\partial_t$ denotes the time derivative, the gradient operator is denoted by $\vec{\nabla} = (\partial_x, \partial_y, \partial_z)$, we use the Einstein sum convention to sum over repeated indices, and the stress tensor $\sigma_{ij}$ is given by

$$\sigma_{ij} = -P\delta_{ij} + \eta(\partial_i v_j + \partial_j v_i), \tag{S2}$$

with $\eta$ the shear viscosity and $P$ the pressure. We assume the medium to be incompressible,

$$\vec{\nabla} \cdot \vec{v} \equiv 0, \tag{S3}$$

and consider gravitational acceleration $F_j = -\delta_{jz} g\rho$ as external force.

Equations (S1), (S3) constitute four equations for the four unknowns $(\vec{v}, P)$. Direct substitution shows that a stationary solution is given by the fluid at rest,

$$\vec{v}^{\,(0)}(\vec{r}) = 0, \tag{S4}$$

$$P^{(0)}(\vec{r}) = P_0 - \rho g z, \tag{S5}$$

where $P_0$ is the pressure at $z = 0$. We consider perturbations $\vec{v}^{(1)}$, $P^{(1)}$ around this stationary solution, i.e. we consider velocity and pressure fields

$$\vec{v}(\vec{r}, t) = \vec{v}^{\,(0)} + \vec{v}^{\,(1)}(\vec{r}, t), \tag{S6}$$

$$P(\vec{r}, t) = P^{(0)}(\vec{r}) + P^{(1)}(\vec{r}, t). \tag{S7}$$

Substitution of eqs. (S6), (S7) into eqs. (S1), (S3) yields

$$\rho\, \partial_t \vec{v}^{\,(1)} = -\vec{\nabla} P^{(1)} + \eta \Delta \vec{v}^{\,(1)}, \tag{S8}$$

$$\vec{\nabla} \cdot \vec{v}^{\,(1)} = 0, \tag{S9}$$

where $\Delta = \partial_x^2 + \partial_y^2 + \partial_z^2$ denotes the Laplace operator. Since $\vec{v}^{\,(0)} = 0$, we have $\vec{v} \equiv \vec{v}^{\,(1)}$ and therefore will omit the superscript "(1)" for the velocity field perturbation in the following.

If the fluid only undergoes small displacements, the velocity field can be written as time derivative of the displacement field $\vec{u}(\vec{r}, t)$ as [2]

$$\vec{v} = \partial_t \vec{u}. \tag{S10}$$

In line with the ansatz we will use in sect. S I C for the displacement field, we assume $\vec{u}$ to be of the form

$$\vec{u} = \vec{\nabla}\Phi + \vec{\nabla} \times \vec{\Psi}, \tag{S11}$$

where $\Phi$, $\Psi$ are potentials for the longitudinal (curl free) and transversal (divergence free) part of the displacement field. Equations (S8), (S9) are then fulfilled if the potentials fulfill

$$\Delta\Phi = 0, \tag{S12}$$

$$\eta \Delta \vec{\Psi} = \rho \partial_t \vec{\Psi}, \tag{S13}$$

and the pressure perturbation is given in terms of the potentials by

$$P^{(1)} = -\rho \partial_t^2 \Phi. \tag{S14}$$

### B. Stress boundary conditions for a viscoelastic interface

A detailed derivation of the continuum mechanical boundary conditions for two bulk media separated by a viscoelastic interface was given by Kralchevsky et. al. [3]. In plane, they assumed the interface to have a purely viscous shear response with viscosity $\eta_{2\mathrm{D}}$, a viscoelastic response to dilation with viscosity $\eta'_{2\mathrm{D}}$ and a position dependent surface tension $\sigma_{2\mathrm{D}}$. For out of plane deformations, they assumed a bending rigidity $\kappa_{2D}$ and a transverse viscosity $\eta^{\perp}_{2\mathrm{D}}$. Furthermore, they considered the

interface to have an area mass density $\rho_{2\mathrm{D}}$ and included an external force per area $\vec{f}_s$ acting on the surface. To linear order in the surface velocity $\vec{v}_{2\mathrm{D}}$, they obtained [4]

$$\rho_{2\mathrm{D}}\partial_t v_{2\mathrm{D},\alpha} = (\sigma_{\mathrm{III},n\alpha} - \sigma_{n\alpha}) + \rho_{2\mathrm{D}} f_{s,\alpha} + \left(\vec{\nabla}_s\right)_\alpha \sigma_{2\mathrm{D}} + \eta'_{2\mathrm{D}} \left(\vec{\nabla}_s\right)_\alpha \left(\vec{\nabla}_s \cdot \vec{v}_{2\mathrm{D}}\right) + \eta_{2\mathrm{D}} \vec{\nabla}_s^2 v_{2\mathrm{D},\alpha} \qquad \alpha \in \{x, y\}, \tag{S15}$$

$$\rho_{2\mathrm{D}}\partial_t v_{2\mathrm{D},n} = (\sigma_{\mathrm{III},nn} - \sigma_{nn}) + \rho_{2\mathrm{D}} f_{s,n} + \sigma_{2\mathrm{D}} \vec{\nabla}_s^2 u_{2\mathrm{D},z} - \kappa_{2D} \vec{\nabla}_s^2 \vec{\nabla}_s^2 u_{2\mathrm{D},z} + \eta_{2\mathrm{D}}^{\perp} \vec{\nabla}_s^2 \partial_t u_{2\mathrm{D},z}, \tag{S16}$$

where $u_{2\mathrm{D},z} \equiv u_{2\mathrm{D},z}(x, y, t)$ is the displacement of the surface point $(x, y, 0)$ in $z$-direction, the stress tensors $\sigma$, $\sigma_{\mathrm{III}}$ for the bulk media below and above the surface are understood to be evaluated at $z = 0$, and $\vec{\nabla}_s := \vec{\nabla} - \hat{n}\left(\hat{n} \cdot \vec{\nabla}\right)$ is the projection of the gradient onto the surface, with $\hat{n}$ the unit normal vector pointing into the $z > 0$ half space. The indices $\alpha$, $n$ label tensor components parallel and perpendicular to the surface, respectively. More generally, we will use the convention that greek indices run over $\{x, y\}$, while latin indices run over $\{x, y, z\}$. For the half-space $z > 0$, we will not consider any dynamics and assume that there is a constant pressure $P_{\mathrm{III}}$, so that

$$\sigma_{\mathrm{III},jk} = -P_{\mathrm{III}}\delta_{jk}. \tag{S17}$$

To rewrite the boundary conditions (S15), (S16), in a form more useful for the present context, we will now relate the surface velocity to the surface displacement, explicitly evaluate $\vec{\nabla}_s$ and use gravitation as external force. This will lead to the expressions eqs. (S25), (S26) for the boundary conditions. To derive an explicit form for the boundary conditions in the linear regime, we will then further rewrite eqs. (S25), (S26) by relating the elastic in-surface dilational response $\sigma_{2\mathrm{D}}$ to the displacement field, leading to eqs. (S31), (S32).

As in the bulk medium, we assume small displacements and approximate the velocity by the time derivative of the displacement,

$$\vec{v}_{2\mathrm{D}} \approx \partial_t \vec{u}_{2\mathrm{D}}, \tag{S18}$$

and furthermore the unit normal vector by the unit vector in $\hat{e}_z$-direction, $\hat{n} \approx \hat{e}_z$. With the latter approximation, we get

$$\vec{\nabla}_s = \hat{e}_x\partial_x + \hat{e}_y\partial_y \equiv \hat{e}_\beta\partial_\beta. \tag{S19}$$

To express $\rho_{2\mathrm{D}}$ in terms of the surface displacement field, we assume that the interfacial area mass density deviates only slightly from its constant equilibrium value, and write

$$\rho_{2\mathrm{D}}(x, y, t) = \rho_{2\mathrm{D}}^{(0)} + \rho_{2\mathrm{D}}^{(1)}(x, y, t), \tag{S20}$$

with $\rho_{2\mathrm{D}}^{(1)}$ small compared to $\rho_{2\mathrm{D}}^{(0)}$. To express $\rho_{2\mathrm{D}}^{(1)}$ in terms of the interfacial displacement field, we integrate the linearized 2D mass conservation equation,

$$\partial_t\rho_{2\mathrm{D}}^{(1)} + \rho_{2\mathrm{D}}^{(0)}\partial_t\partial_\beta u_{2\mathrm{D},\beta} = 0, \tag{S21}$$

with respect to time to get

$$\rho_{2\mathrm{D}}^{(1)} = -\rho_{2\mathrm{D}}^{(0)}\partial_\beta u_{2\mathrm{D},\beta}. \tag{S22}$$

The constant of integration was chosen so that an area preserving deformation, $\partial_\beta u_{2\mathrm{D},\beta} = 0$, implies no area density change, $\rho_{2\mathrm{D}}^{(1)} = 0$. Using eq. (S22) to eliminate $\rho_{2\mathrm{D}}^{(1)}$ in eq. (S20), we obtain

$$\rho_{2\mathrm{D}} = \rho_{2\mathrm{D}}^{(0)}\left(1 - \partial_\beta u_{2\mathrm{D},\beta}\right). \tag{S23}$$

Using this equation, the area force density due to gravitational acceleration is given by

$$\rho_{2\mathrm{D}}\vec{f}_s = -\rho_{2\mathrm{D}} g\vec{e}_z = -\rho_{2\mathrm{D}}^{(0)} g\left(1 - \partial_\beta u_{2\mathrm{D},\beta}\right)\vec{e}_z. \tag{S24}$$

Equation (S24) shows that even if there is no local compression or expansion, $\partial_\beta u_{2\mathrm{D},\beta} = 0$, gravity causes a constant area force density $-\rho_{2\mathrm{D}}^{(0)} g\vec{e}_z$ on the interface. For the equilibrium solution, around which we perturb, the surface should be at rest at $z = 0$. This means that, in the equilibrium solution where there is no displacement, the constant background pressure $P_0$ in the lower bulk medium (c.f. eq. (S5)) and the constant pressure $P_{\mathrm{III}}$ in the upper bulk medium need to differ exactly by the pressure gravitational forces acting on the interface exert on the lower medium in equilibrium, i.e. $P_0 - P_{\mathrm{III}} = \rho_{2\mathrm{D}}^{(0)} g$, so that the interface remains at $z = 0$.

Inserting the expressions for $\vec{v}_{2\mathrm{D}}$, $\vec{\nabla}_s$, $\rho_{2\mathrm{D}}$ and $\rho_{2\mathrm{D}}\vec{f}_s$, namely eqs. (S18), (S19), (S23), (S24), into the boundary conditions (S15), (S16), we obtain

$$\rho_{2\mathrm{D}}^{(0)}\partial_t^2 u_{2\mathrm{D},\alpha} = (\sigma_{\mathrm{III},z\alpha} - \sigma_{z\alpha}) + \partial_\alpha\sigma_{2\mathrm{D}} + \eta'_{2\mathrm{D}}\partial_t\partial_\alpha\partial_\beta u_{2\mathrm{D},\beta} + \eta_{2\mathrm{D}}\partial_t\partial_\beta^2 u_{2\mathrm{D},\alpha} \qquad \alpha \in \{x, y\}, \tag{S25}$$

$$\rho_{2\mathrm{D}}^{(0)}\partial_t^2 u_{2\mathrm{D},z} = (\sigma_{\mathrm{III},zz} - \sigma_{zz}) - \rho_{2\mathrm{D}}^{(0)} g\left(1 - \partial_\beta u_{2\mathrm{D},\beta}\right) + \left(\sigma_{2\mathrm{D}} + \eta_{2\mathrm{D}}^{\perp}\partial_t - \kappa_{2D}\partial_\beta^2\right)\partial_\beta^2 u_{2\mathrm{D},z}. \tag{S26}$$

To express $\sigma_{2\mathrm{D}}$ in terms of the surface displacement, we assume that the surface tension deviates only slightly from its constant equilibrium value, and write

$$\sigma_{2\mathrm{D}}(x, y, t) = \sigma_{2\mathrm{D}}^{(0)} + \sigma_{2\mathrm{D}}^{(1)}(x, y, t), \tag{S27}$$

with $\sigma_{2\mathrm{D}}^{(1)}$ small compared to $\sigma_{2\mathrm{D}}^{(0)}$. To express $\sigma_{2\mathrm{D}}^{(1)}$ in terms of the surface displacement field, we consider the definition of the 2D in-plane elastic modulus $K_{2\mathrm{D}}$,

$$K_{2\mathrm{D}} = a\frac{\partial\sigma_{2\mathrm{D}}}{\partial a}, \tag{S28}$$

which relates local changes in the area per lipid $a$ of a surface element to the local surface tension $\sigma_{2\mathrm{D}}$. Note that, unlike in the analogous equation for the three dimensional bulk modulus, there is no minus sign in eq. (S28) because surface tension can be thought of as negative surface pressure. $K_{2\mathrm{D}}$ not only depends on the material the

interface is made of but also on the thermodynamics of the deformation (e.g. isothermal, adiabatic). Equation (S28) can be integrated to yield

$$\sigma_{2D}^{(1)} = -K_{2D}\partial_\beta u_{2D,\beta}, \tag{S29}$$

where we used $\Delta a/\bar{a} \equiv (a-\bar{a})/\bar{a} = \partial_\beta u_{2D,\beta}$ [5], with $\bar{a}$ the equilibrium area per lipid, and fixed the constant of integration by assuming that no area change implies no surface tension change. Eliminating $\sigma_{2D}^{(1)}$ in eq. (S27) using eq. (S29), we get

$$\sigma_{2D} = \sigma_{2D}^{(0)} - K_{2D}\partial_\beta u_{2D,\beta}, \tag{S30}$$

so that the boundary conditions eqs. (S25), (S26), finally become, to linear order in the interfacial displacement field,

$$\begin{aligned}\rho_{2D}^{(0)}\partial_t^2 u_{2D,\alpha} &= (\sigma_{\mathrm{III},z\alpha} - \sigma_{z\alpha}) + \partial_\alpha\left(K_{2D} + \eta'_{2D}\partial_t\right)\partial_\beta u_{2D,\beta}\\ &\quad + \eta_{2D}\partial_t\partial_\beta^2 u_{2D,\alpha} \qquad \alpha\in\{x,y\}, \end{aligned}\tag{S31}$$

$$\begin{aligned}\rho_{2D}^{(0)}\partial_t^2 u_{2D,z} &= (\sigma_{\mathrm{III},zz} - \sigma_{zz}) - \rho_{2D}^{(0)} g\left(1-\partial_\beta u_{2D,\beta}\right)\\ &\quad + \left(\sigma_{2D}^{(0)} + \eta_{2D}^{\perp}\partial_t - \kappa_{2D}\partial_\beta^2\right)\partial_\beta^2 u_{2D,z}.\end{aligned}\tag{S32}$$

Since the perturbations $\rho_{2D}^{(1)}$, $\sigma_{2D}^{(1)}$ do not appear explicitly in eqs. (S31), (S32) anymore, we will drop the superscripts (0) of the corresponding equilibrium values $\rho_{2D}^{(0)}$, $\sigma_{2D}^{(0)}$ in the following, and have also dropped them in the main text.

### C. Harmonic wave ansatz and implicit dispersion relation

To solve eqs. (S8), (S9) with boundary conditions eqs. (S31), (S32), we use a harmonic wave ansatz [6] for the displacement potentials that were introduced in eq. (S11),

$$\Phi(\vec{r},t) = \phi e^{z/\lambda_l} e^{i(kx-\omega t)}, \tag{S33}$$

$$\vec{\Psi}(\vec{r},t) = \hat{e}_y \psi e^{z/\lambda_t} e^{i(kx-\omega t)}, \tag{S34}$$

where we assume $\mathrm{Re}(k) > 0$, so that the wave propagates in the positive $x$-direction. According to eq. (S11), the resulting displacmenet field is given by

$$\vec{u}(\vec{r},t) = \left[\begin{pmatrix} ik \\ 0 \\ \lambda_l^{-1}\end{pmatrix}\phi e^{z/\lambda_l} + \begin{pmatrix} -\lambda_t^{-1} \\ 0 \\ ik\end{pmatrix}\psi e^{z/\lambda_t}\right] e^{i(kx-\omega t)}, \tag{S35}$$

so that according to eq. (S10), we obtain the velocity field

$$\vec{v}(\vec{r},t) = (-i\omega)\left[\begin{pmatrix} ik \\ 0 \\ \lambda_l^{-1}\end{pmatrix}\phi e^{z/\lambda_l} + \begin{pmatrix} -\lambda_t^{-1} \\ 0 \\ ik\end{pmatrix}\psi e^{z/\lambda_t}\right] e^{i(kx-\omega t)}. \tag{S36}$$

The harmonic wave ansatz contains 6 parameters: $k$, $\omega$, $\phi$, $\psi$, $\lambda_l$, $\lambda_t$. We assume $\omega \in \mathbb{R}$, and $\omega > 0$ is a given constant, i.e. we consider waves of frequency $\omega$ and want to obtain the corresponding wavenumber $k(\omega)$. The constants $\lambda_l$, $\lambda_t$ are determined by substituting eqs. (S33), (S34), into eqs. (S12), (S13), which yields

$$\lambda_l^{-2} = k^2, \tag{S37}$$

$$\lambda_t^{-2} = k^2 + \frac{-i\omega\rho}{\eta}. \tag{S38}$$

Because the physical assumption that the wave decays as $z \to -\infty$ requires $\mathrm{Re}(\lambda_l^{-1})$, $\mathrm{Re}(\lambda_t^{-1}) > 0$, eqs. (S37), (S38) determine $\lambda_l$, $\lambda_t$ uniquely as a function of $k$, $\omega$, since the complex square root with positive real part has to be chosen. The stress boundary conditions eqs. (S31), (S32) at $z = 0$ yield a homogeneous linear system of two equations for the two coefficients $\phi$, $\psi$. This system can be obtained explicitly by calculating $\sigma_{ij}$, $u_{2D,i} \equiv u_i|_{z=0}$, for the displacement field eq. (S35) and the stress strain relation eq. (S2), and then substituting these into the boundary conditions eqs. (S31), (S32) (for (S31), only the $\alpha = 1$ case is needed, since for $\alpha = 2$ the equation is fulfilled trivially, as a short calculation shows). The stress boundary conditions then become

$$\begin{aligned}0 &= ik\left[\, i\omega\rho_{2D} - k^2\tilde{g}_{2D} - 2\eta k \,\right]\phi \\ &\quad + \left[\,\lambda_t^{-1}(k^2\tilde{g}_{2D} - i\omega\rho_{2D}) + \eta(k^2+\lambda_t^{-2})\,\right]\psi,\end{aligned}\tag{S39}$$

$$\begin{aligned}0 &= \left[\, k(\omega^2\rho_{2D} - k^2\tilde{\Pi}_{2D} - \rho g) - k^2\rho_{2D} g + i\omega\eta(k^2+\lambda_t^{-2})\,\right]\phi \\ &\quad + ik\left[\,\omega^2\rho_{2D} - k^2\tilde{\Pi}_{2D} - \lambda_t^{-1}\rho_{2D} g - \rho g + i\omega 2\eta\lambda_t^{-1}\,\right]\psi,\end{aligned}\tag{S40}$$

where again $\lambda_t$ is given by eq. (S38), and the response functions $\tilde{g}_{2D}$, $\tilde{\Pi}_{2D}$ are given by

$$\tilde{g}_{2D}(\omega) := \eta_{2D} + \eta'_{2D} + K_{2D}/(-i\omega), \tag{S41}$$

$$\tilde{\Pi}_{2D}(k,\omega) := \sigma_{2D} + (-i\omega)\eta_{2D}^{\perp} + k^2\kappa_{2D}. \tag{S42}$$

In order to have a propagating wave with nonzero amplitude, the eqs. (S39), (S40) need to have a nontrivial solution for $\phi$, $\psi$. Consequently, the implicit dispersion relation is obtained by setting the determinant of the $2\times 2$ coefficient matrix for $\phi$, $\psi$, obtained from eqs. (S39), (S40), equal to zero. This leads to

$$\begin{aligned}0 &= k\left(k^2\tilde{\Pi}_{2D} + \rho g - \omega^2\rho_{2D}\right)\\ &\qquad \times\left[\left(k^2\tilde{g}_{2D} - i\omega\rho_{2D}\right)\left(k - \lambda_t^{-1}\right) + i\omega\rho\right]\\ &\quad + \left(k^2\tilde{g}_{2D} - i\omega\rho_{2D}\right)\omega^2\rho\lambda_t^{-1}\\ &\quad + \eta\left[\, i\omega\eta\left(-4k^2\lambda_l^{-1}\lambda_t^{-1} + (k^2+\lambda_t^{-2})^2\right)\right.\\ &\qquad \left. - \rho_{2D} g k^2\left(k-\lambda_t^{-1}\right)^2\,\right].\end{aligned}\tag{S43}$$

A solution $k(\omega)$ to eq. (S43) yields the dispersion relation of a surface wave, for which phase velocity and propagation distance can then be calculated via

$$c_{\|}(\omega) = \frac{\omega}{\mathrm{Re}(k(\omega))}, \quad \text{(S44)}$$

$$\lambda_{\|}(\omega) = \frac{1}{\mathrm{Im}(k(\omega))}. \quad \text{(S45)}$$

### D. Factorization of the implicit dispersion relation and Lucassen dispersion relation

As it stands, eq. (S43) is too complicated to be solved analytically. However, under certain conditions, which as we will see in sect. S I E are appropriate for the surface waves we are interested in, approximate analytical solutions can be obtained:

Assuming

$$\frac{\rho|\omega|}{\eta|k|^2} \gg 1, \quad \text{(S46)}$$

we have

$$\lambda_t^{-2} \approx -i\omega\rho/\eta, \quad \text{(S47)}$$

c.f. eq. (S38), and $|\lambda_t^{-1}| \gg |k|$, so that eq. (S43) simplifies to

$$\begin{aligned} 0 = k &\left(k^2\tilde{\Pi}_{2D} + \rho g - \omega^2\rho_{2D}\right) \\ &\times \left[\left(k^2\tilde{g}_{2D} - i\omega\rho_{2D}\right)\left(k - \lambda_t^{-1}\right) + i\omega\rho\right] \\ &+ \left(k^2\tilde{g}_{2D} - i\omega\rho_{2D}\right)\omega^2\rho\lambda_t^{-1} \\ &- i\omega\rho\left(\omega^2\rho - \rho_{2D}gk^2\right). \end{aligned} \quad \text{(S48)}$$

Furthermore assuming that the gravitational force on the interface can be neglected,

$$\rho_{2D}g \ll \frac{\rho|\omega|^2}{|k|^2}, \quad \text{(S49)}$$

eq. (S48) factorizes to yield

$$\begin{aligned} 0 = &\left[k\left(k^2\tilde{\Pi}_{2D} + \rho g - \omega^2\rho_{2D}\right) - \rho\omega^2\right] \\ &\times \left[\left(k^2\tilde{g}_{2D} - i\omega\rho_{2D}\right)\lambda_t^{-1} - i\omega\rho\right], \end{aligned} \quad \text{(S50)}$$

and one obtains the two independent dispersion relations

$$0 = k\left(k^2\tilde{\Pi}_{2D} + \rho g - \omega^2\rho_{2D}\right) - \rho\omega^2, \quad \text{(S51)}$$

$$0 = \left(k^2\tilde{g}_{2D} - i\omega\rho_{2D}\right)\sqrt{(-i\omega\rho)/\eta} - i\omega\rho, \quad \text{(S52)}$$

where we used eq. (S47) and the square root is the complex root with positive real part. Whether a solution $k(\omega)$ of eqs. (S51), (S52) fulfills the factorization conditions eqs. (S46), (S49), can of course only be checked a posteriori, i.e. once a solution $k(\omega)$ has been obtained, because $k$ appears in both inequalities.

Equation (S51) is a generalization of the standard capillary-gravity wave dispersion relation [2, 7], and additionally includes the inertia of the interface, as well as surface viscosity and bending rigidity of the interface via $\tilde{\Pi}_{2D}$, c.f. eq. (S42). Equation (S52) is a generalization of the Lucassen dispersion relation [6, 8], and additionally includes the inertia of the interface. To obtain the classic Lucassen dispersion relation, we first note that eq. (S52) can immediately be solved for $k^2$, to yield

$$k^2 = \frac{i\omega}{\tilde{g}_{2D}}\left(\sqrt{\frac{\rho\eta}{-i\omega}} + \rho_{2D}\right). \quad \text{(S53)}$$

If the inertia of the interface can be neglected,

$$|\rho_{2D}| \ll \left|\sqrt{\frac{\rho\eta}{-i\omega}}\right|, \quad \text{(S54)}$$

eq. (S53) simplies to

$$k^2 = \frac{i\omega}{\tilde{g}_{2D}}\sqrt{\frac{\rho\eta}{-i\omega}}. \quad \text{(S55)}$$

If furthermore the interfacial response is purely elastic,

$$\tilde{g}_{2D}(\omega) = \eta_{2D} + \frac{K_{2D}}{-i\omega} \approx \frac{K_{2D}}{-i\omega}, \quad \text{(S56)}$$

eq. (S57) further simplifies to

$$k^2 = \frac{\omega^2}{K_{2D}}\sqrt{\frac{\rho\eta}{-i\omega}}, \quad \text{(S57)}$$

which finally leads to

$$k(\omega) = e^{i\pi/8}\sqrt{\frac{\sqrt{\rho\eta\omega^3}}{K_{2D}}}, \quad \text{(S58)}$$

where we choose the complex square root that leads to a positive real part for $k$, so that the resulting wave propagates in the positive $\hat{e}_x$-direction. This approximate solution of eq. (S52), valid as long as eqs. (S54), (S56) are fulfilled, is the classical Lucassen dispersion relation [6].

### E. Discussion of the factorization conditions for Lucassen waves in a lipid monolayer on water

In the previous subsection we showed that the derivation of the classical Lucassen dispersion relation, eq. (S58) from the full implicit dispersion relation eq. (S43) rests on four approximations, namely eqs. (S46), (S49), (S54), (S56). We now show that for a DPPC monolayer on water, there is a frequency range spanning 10 orders of magnitude and including the frequency range relevant to us, where these approximations are justified.

More explicitly, we consider the parameters

$$\eta = 10^{-3}\ \mathrm{Pa \cdot s}, \quad \text{(S59)}$$

$$\rho = 10^3\ \mathrm{kg/m^3}, \quad \text{(S60)}$$

$$g = 9.81\ \mathrm{m/s^2}, \quad \text{(S61)}$$

appropriate for water as bulk medium [9] and standard gravitational acceleration, and the interface parameters

$$\rho_{2\mathrm{D}} = 1 \cdot 10^{-6}\ \mathrm{kg/m^2}, \tag{S62}$$
$$\eta_{2\mathrm{D}} = 1 \cdot 10^{-9}\ \mathrm{Pa \cdot s \cdot m}, \tag{S63}$$
$$\eta'_{2\mathrm{D}} = 0, \tag{S64}$$
$$\eta^{\perp}_{2\mathrm{D}} = 1 \cdot 10^{-9}\ \mathrm{Pa \cdot s \cdot m}, \tag{S65}$$
$$K_{2\mathrm{D}} = 1 \cdot 10^{-2}\ \mathrm{N/m}, \tag{S66}$$
$$\sigma_{2\mathrm{D}} = 7 \cdot 10^{-2}\ \mathrm{N/m}, \tag{S67}$$
$$\kappa_{2D} = 3 \cdot 10^{-19}\ \mathrm{N \cdot m}, \tag{S68}$$

appropriate for a DPPC monolayer. The values for $\sigma_{2\mathrm{D}}$, $K_{2\mathrm{D}}$ can be obtained via measuring Langmuir isotherms [10, 11], the shear viscosity $\eta_{2\mathrm{D}}$ for a DPPC bilayer can be measured by observing diffusion in lipid membranes [12, 13], while the bending rigidity $\kappa_{2D}$ can be measured via weakly deforming bilayer vesicles [14, 15].

Using these parameters and the solution eq. (S58), eqs. (S46), (S49), (S54), (S56) become, respectively,

$$\text{eq. (S46)} \iff \omega \ll \frac{K_{2\mathrm{D}}^2 \rho}{\eta^3} = 10^{10}\frac{1}{\mathrm{s}}, \tag{S69}$$
$$\text{eq. (S49)} \iff \omega \gg \frac{\eta \rho_{2\mathrm{D}}^2 g^2}{\rho K_{2\mathrm{D}}} \approx 10^{-3}\frac{1}{\mathrm{s}}, \tag{S70}$$
$$\text{eq. (S54)} \iff \omega \ll \frac{\rho\eta}{\rho_{2\mathrm{D}}^2} = 10^{12}\frac{1}{\mathrm{s}}, \tag{S71}$$
$$\text{eq. (S56)} \iff \omega \ll \frac{K_{2\mathrm{D}}}{\eta_{2\mathrm{D}}} = 10^{7}\frac{1}{\mathrm{s}}. \tag{S72}$$

Thus, for frequencies

$$10^{-3}\frac{1}{\mathrm{s}} \ll \omega \ll 10^{7}\frac{1}{\mathrm{s}}, \tag{S73}$$

eq. (S58), an approximate solution to the implicit dispersion relation eq. (S43), is self-consistent with the approximations used to derive it. In particular, since we are interested in dynamics on the millisecond time scale, $\omega \approx 10^3$ 1/s, this frequency range includes the regime of interest to us.

In fig. S2, we supplement our analytical estimates by a plot of the phase velocities and propagation distances for both the approximate solution eq. (S58) and the corresponding numerical solution of the full implicit dispersion relation, eq. (S43). Consistent with eq. (S73), the two solutions $k(\omega)$ lead to basically identical wave properties for frequencies up to $\omega \approx 10^6$ 1/s.

### F. Identification of the dominating term in the displacement field of the Lucassen wave

As discussed in sect. S I C, the displacement field of the Lucassen wave has components in the $\hat{e}_x$ and $\hat{e}_z$ direction. More explicitly, it is given by eq. (S35) with $\lambda_l^{-1} = k$,

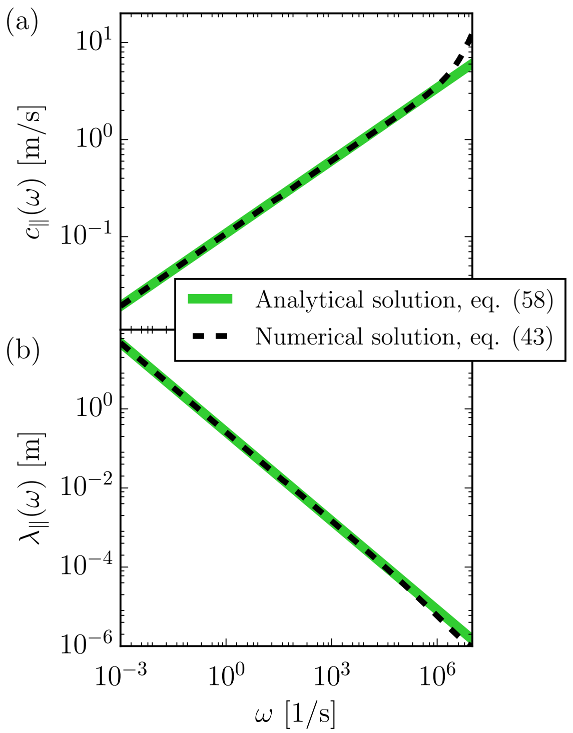


FIG. S2. **Comparison of analytical Lucassen relation to numerical solution of full implicit dispersion relation.** The black dashed line shows the numerical solution to eq. (S43) corresponding to the Lucassen wave, while the green solid line shows the approximate analytical Lucassen dispersion relation, eq. (S58). Phase velocities and propagation distances are calculated using eqs. (S44), (S45).

$\lambda_t^{-1} = \sqrt{(-i\omega\rho)/\eta}$, c.f. eqs. (S37), (S47), as

$$\vec{u}(\vec{r},t) = (\vec{\nabla}\Phi)(\vec{r},t) + (\vec{\nabla}\times\vec{\Psi})(\vec{r},t) = \tag{S74}$$
$$= \left[\phi \begin{pmatrix} ik \\ 0 \\ k \end{pmatrix} e^{kz} + \psi \begin{pmatrix} -\lambda_t^{-1} \\ 0 \\ ik \end{pmatrix} e^{z/\lambda_t}\right] e^{i(kx-\omega t)}, \tag{S75}$$

with $k$ given by eq. (S58).

To determine which component of the displacement field is dominant, we compare the magnitudes of all components of both the longitudinal and transversal parts to each other, i.e. we compare $|\hat{e}_x \cdot (\vec{\nabla}\Phi)|$, $|\hat{e}_z \cdot (\vec{\nabla}\Phi)|$, $|\hat{e}_x \cdot (\vec{\nabla}\times\vec{\Psi})|$, $|\hat{e}_z \cdot (\vec{\nabla}\times\vec{\Psi})|$. We discuss this situation for the displacement field at the interface ($z = 0$) of an elastic membrane on water, i.e. we consider the parameters from sect. S I E, eqs. (S59-S68).

From eq. (S75) it can immediately be read off that $|\hat{e}_x \cdot (\vec{\nabla}\Phi)|$, $|\hat{e}_z \cdot (\vec{\nabla}\Phi)|$ have the same order of magnitude, namely $|\phi k|$. On the other hand, as shown in sect. S I D, for $\omega \ll 10^7$ 1/s, $|\lambda_t^{-1}| \gg |k|$, so that $|\hat{e}_x \cdot (\vec{\nabla}\times\vec{\Psi})| \gg |\hat{e}_z \cdot (\vec{\nabla}\times\vec{\Psi})|$.

Now to compare $|\hat{e}_i \cdot (\vec{\nabla}\Phi)|$, $|\hat{e}_1 \cdot (\vec{\nabla}\times\vec{\Psi})|$, we need an order-of-magnitude estimate for $|\phi/\psi|$. This relative am-

plitude can be obtained by solving any of the boundary condition eqs. (S39), (S40) for $\phi/\psi$. We solve eq. (S39) for $\phi/\psi$ and use the numerical solution of eq. (S43) corresponding to the Lucassen wave for $k(\omega)$, to calculate the fraction $|\phi/\psi|$ numerically as a function of frequency $\omega$. The result is shown in fig. S3 (a). As can be seen there, for frequencies $10^{-3}$ 1/s $< \omega <$ $10^{7}$ 1/s, it holds that

$$0.1 < \left|\frac{\phi}{\psi}\right| < 10, \tag{S76}$$

so that $|\phi|$, $|\psi|$ are of the same order of magnitude. Thus, since according to eq. (S46) $|\lambda_t^{-1}| \gg |k|$, we have $|\phi k| \ll |\psi\lambda_t^{-1}|$, and therefore $|\hat{e}_x \cdot (\vec{\nabla} \times \vec{\Psi})| \gg |\hat{e}_i \cdot (\vec{\nabla}\Phi)|$, $i \in \{x, z\}$.

In summary, for frequencies $10^{-3}$ 1/s $< \omega <$ $10^{7}$ 1/s, the displacement field for the Lucassen wave is at the interface $z = 0$ dominated by the $\hat{e}_x$ component of $\vec{\nabla} \times \vec{\Psi}$, and thus approximately given by

$$\vec{u}(x, z = 0, t) \approx -\hat{e}_x \psi \lambda_t^{-1} e^{i(kx - \omega t)}. \tag{S77}$$

In accordance with these estimates, we show in fig. S3 (b) plots of $|k\phi|$, $|k\psi|$, $|\lambda_t^{-1}\psi|$, representing the components we just compared, with $k$ the numerical solution of eq. (S43) corresponding to the Lucassen wave, $\phi = 1$ m$^2$ and $\psi$ as calculated from eq. (S39). The term $|\lambda_t^{-1}\psi|$, which according to eq. (S75) gives the order of magnitude of the $\hat{e}_x$ component of $\vec{\nabla} \times \vec{\Psi}$, is indeed the largest term.

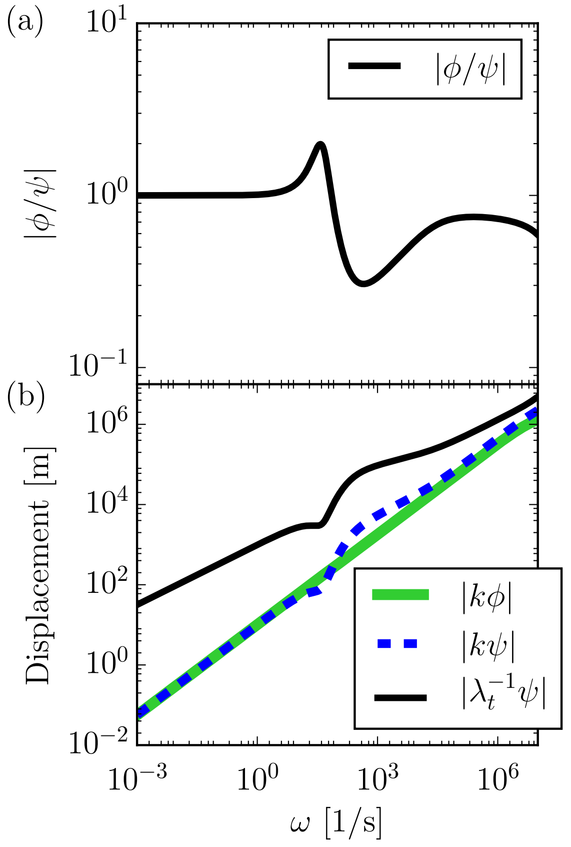


FIG. S3. **(a): Relative magnitude of the coefficients $\phi$, $\psi$ of longitudinal and transversal parts of the harmonic wave ansatz.** The boundary condition (S39) is solved for $\phi/\psi$, and using $k(\omega)$ from a numerical solution of eq. (S43) for the parameters from sect. S I E, $|\phi/\psi|$ is calculated as a function of $\omega$; **(b): Absolute values of the individual vector components of longitudinal and transversal parts of the harmonic wave ansatz.** Using $k(\omega)$ obtained from numerically solving eq. (S43), $\lambda_t$ as given by eq. (S38), $\phi/\psi$ as obtained by solving eq. (S39) for $\phi/\psi$, and setting $\phi = 1$ m$^2$, the quantities $|k\psi|$, $|k\psi|$, $|\lambda_t^{-1}\psi|$ are calculated as a function of $\omega$. According to eq. (S75), the plotted curves correspond to the magnitudes of the individual terms appearing in the surface wave displacement field. Note that in the context of linear theory, the choice $\phi = 1$ m$^2$ simply sets a scale, and only the relative sizes of the terms plotted here are of relevance for determining the dominant component of the displacement field.

## S II. DIRECT DERIVATION OF THE FRACTIONAL WAVE EQUATION FROM MOMENTUM CONSERVATION AND STRESS BOUNDARY CONDITIONS

In the main text, we introduce the fractional wave equation based on the Lucassen dispersion relation and the fact that the corresponding interfacial displacement is dominated by the $\hat{e}_x$-component, c.f. sect. S I. In this section, we give a derivation of the fractional wave equation directly from momentum conservation in the bulk medium $z < 0$ and the stress boundary condition at the interface $z = 0$.

As already mentioned in sect. S I, a stationary solution of the linearlized Navier-Stokes equation (S1) for an incompressible medium under the influence of gravity, $\vec{F} = -\hat{e}_z \rho g$, is given by the fluid at rest, with velocity and pressure fields

$$\vec{v}^{\,(0)}(\vec{r}) = 0, \tag{S78}$$

$$P^{(0)}(\vec{r}) = P_0 - \rho g z, \tag{S79}$$

with $P_0$ the pressure at $z = 0$. As in the derivation of the Lucassen dispersion relation, we consider perturbations $\vec{v}^{\,(1)}$, $P^{(1)}$ around this solution, i.e. we consider velocity and pressure fields

$$\vec{v}(\vec{r}, t) = \vec{v}^{\,(0)} + \vec{v}^{\,(1)}(\vec{r}, t), \tag{S80}$$

$$P(\vec{r}, t) = P^{(0)}(\vec{r}) + P^{(1)}(\vec{r}, t). \tag{S81}$$

Substitution of these into momentum conservation, eq. (S1), and the incompressibility condition, eq. (S3), yields

$$\rho \partial_t \vec{v}^{\,(1)} = -\vec{\nabla} P^{(1)} + \eta \Delta \vec{v}^{\,(1)}, \tag{S82}$$

$$\vec{\nabla} \cdot \vec{v}^{\,(1)} = 0, \tag{S83}$$

which are the linearized equations for incompressible Newtonian fluids with constant density and without external forces. Since $\vec{v}^{\,(0)} = 0$, we have $\vec{v} \equiv \vec{v}^{\,(1)}$ and will therefore omit the superscript "(1)" for the velocity field

perturbation in the following.

Assuming a displacement field of the form

$$\vec{u}(\vec{r},t) = \begin{pmatrix} u_x(x,z,t) \\ 0 \\ u_z(x,z,t) \end{pmatrix}, \tag{S84}$$

appropriate for a wavefront travling in the $\hat{e}_x$-direction, and assuming that the pressure only depends on the distance from the interface, $P^{(1)}(\vec{r},t) \equiv P^{(1)}(z,t)$, momentum conservation in the $\hat{e}_x$ direction, eq. (S82) with $i = x$, becomes

$$\rho \partial_t^2 u_x = \eta \Delta \partial_t u_x, \tag{S85}$$

where we used that for small displacements $\partial_t \vec{u} \approx \vec{v}$. Assuming that the right hand side of this equation is dominated by the velocity gradient away from the interface,

$$\Delta \partial_t u_x = \left(\partial_x^2 + \partial_z^2\right) \partial_t u_x \approx \partial_z^2 \partial_t u_x \tag{S86}$$

which physically we associate with the velocity of the surface wave varying on a much shorter length scale away from the interface than in the direction of propagation, eq. (S85) becomes

$$\rho \partial_t^2 u_x = \eta \partial_t \partial_z^2 u_x. \tag{S87}$$

Integrating this equation with respect to time and dividing by $\eta$ leads to

$$\frac{\rho}{\eta} \partial_t u_x = \partial_z^2 u_x, \tag{S88}$$

where we chose the constant of integration such that no spatial change in stress implies no temporal change in displacement. Formally taking the square root of the differential operators on both sides of eq. (S88) yields

$$\sqrt{\frac{\rho}{\eta}} \partial_t^{1/2} u_x = \partial_z u_x. \tag{S89}$$

Now as for the stress boundary condition at $z = 0$, the $\alpha = x$ component of the stress boundary condition eq. (S25) for an interface with negligible interfacial viscosities is

$$\rho_{2\mathrm{D}} \partial_t^2 U = \left(\sigma_{\mathrm{III},z\alpha} - \sigma_{z\alpha}\right)\big|_{z=0} + \partial_x \sigma_{2\mathrm{D}}, \tag{S90}$$

where $\rho_{2\mathrm{D}}$ is the equilibrium area mass density of the interface, $U(x,t) \equiv u_x(x, z=0, t)$ is the interfacial displacement in the $\hat{e}_x$-direction, $\sigma_{\mathrm{III}}$, $\sigma$ are the stress tensors of the bulk medium above and below the interface, and $\sigma_{2\mathrm{D}}$ is the surface tension of the interface. Note that, as opposed to eq. (S25), we have dropped the superscript "(0)" of the equilibrium membrane area mass density $\rho_{2\mathrm{D}}^{(0)}$ here.

We now rewrite the term $\partial_x \sigma_{2\mathrm{D}}$ on the right hand side of eq. (S99). For this, first note that the surface tension $\sigma_{2\mathrm{D}}$ is just the negative interfacial pressure $\pi$, so that

$$\sigma_{2\mathrm{D}}(a) = -\pi(a), \tag{S91}$$

with $a$ the area per lipid (or more generally area per molecule). For a given equilibrium area per lipid $\bar{a}$, the actual area per lipid can be written in terms of the relative area change

$$\Delta a/\bar{a} := \frac{a - \bar{a}}{\bar{a}} \tag{S92}$$

as

$$a = \bar{a}\left(1 + \Delta a/\bar{a}\right), \tag{S93}$$

which follows immediately from solving eq. (S92) for $a$. Using eqs. (S91), (S93) and the chain rule, we calculate

$$\partial_x \sigma_{2\mathrm{D}} = -\partial_x \pi = -(\partial_a \pi)\partial_x a = -(\partial_a \pi)\, \bar{a}\, \partial_x(\Delta a/\bar{a}). \tag{S94}$$

To simplify this expression, we note that the elastic modulus $K_{2\mathrm{D}}$ (the inverse of the compressibility) of the interface is defined by

$$K_{2\mathrm{D}} = -a \partial_a \pi, \tag{S95}$$

and that the local relative area change is given in terms of the interfacial displacement field as [5]

$$\Delta a/\bar{a} = \partial_\beta u_{2\mathrm{D},\beta}\big|_{z=0} = \partial_x U, \tag{S96}$$

where at the last equality sign we used our assumption of no displacement in the $\hat{e}_y$-direction, c.f. eq. (S84). Using eqs. (S95), (S96), eq. (S94) can then be rewritten as

$$\partial_x \sigma_{2\mathrm{D}} = -(\partial_a \pi)\, \bar{a}\, \partial_x(\Delta a/\bar{a}) = -a\, (\partial_a \pi)\, \bar{a}/a\, \partial_x^2 U \tag{S97}$$

$$= \frac{K_{2\mathrm{D}}}{1 + \partial_x U}\, \partial_x^2 U, \tag{S98}$$

where at the last equality sign we used $\bar{a}/a = 1/(1 + \Delta a/\bar{a}) = 1/(1 + \partial_x U)$, c.f. eqs. (S92), (S96).

As we will justify in sect. S IV, we neglect nonlinear effects caused by the factor $1/(1+\partial_x U)$, so that eq. (S98) allows us to rewrite the boundary condition (S99) as

$$\rho_{2\mathrm{D}} \partial_t^2 U = \left(\sigma_{\mathrm{III},z\alpha} - \sigma_{z\alpha}\right)\big|_{z=0} + K_{2\mathrm{D}} \partial_x^2 U. \tag{S99}$$

If we now assume again that the velocities change on a smaller length scale away from the interface than in the direction of propagation, c.f. eq. (S86), and that dynamical stresses from the upper half space $z > 0$ can be neglected, we can approximate the bulk media stresses as

$$\left(\sigma_{\mathrm{III},zx} - \sigma_{zx}\right)\big|_{z=0} = -\eta\, \left(\partial_x v_z + \partial_z v_x\right)\big|_{z=0} \approx -\eta \partial_z\, v_x\big|_{z=0}$$

$$= -\eta \partial_t \partial_z\, u_x\big|_{z=0}\,. \tag{S100}$$

Inserting this into eq. (S99) and replacing $\partial_z u_x|_{z=0}$ using eq. (S89), the boundary condition eq. (S99) finally becomes

$$\rho_{2\mathrm{D}} \partial_t^2 U = -\sqrt{\eta\rho}\, \partial_t^{3/2} U + K_{2\mathrm{D}}\, \partial_x^2 U, \tag{S101}$$

which is the fractional wave equation we use in the main text. It is derived here as an approximate stress boundary condition at the interface, and momentum conservation has been used to eliminate the derivative $\partial_z$, so that the equation could be expressed solely in terms of the displacement field $\vec{u}$ at $z=0$ and its spatial derivatives in the $\hat{e}_x$-direction, i.e. along the interface. The two approximations used here, eqs. (S86), (S100), are of course motivated by the properties of the Lucassen wave discussed in sect. S I.

We note that with the present derivation, it is immediately clear how one could include the membrane shear viscosity in the derivation: One would simply not neglect the corresponding terms in the boundary condition, eq. (S31).

As a final remark, we note that the interfacial displacement in the $\hat{e}_z$-direction, $u_{2\mathrm{D},z}(x, z=0, t)$, can be calculated from a solution of eq. (S101): After solving eq. (S101), the resulting $U(x,t) \equiv u_{2\mathrm{D},x}(x, z=0, t)$ can be considered as inhomogeneity in the remaining boundary condition, eq. (S32), which can then be solved to obtain the corresponding displacement field $u_{2\mathrm{D},z}(x, z=0, t)$.

## S III. NUMERICAL DETAILS FOR THE CALCULATION OF THE ELASTIC MODULUS $K_{2\mathrm{D}}$

In this section, we discuss details of the calculation of the experimental isothermal elastic modulus $K_{2\mathrm{D}}$. Experimentally, a Langmuir isotherm $\pi(a)$, with $\pi$ the surface pressure and $a$ the area per lipid, is measured for a DPPC monolayer on water. The isothermal elastic modulus is then given by

$$K_{2\mathrm{D}} = -a\left(\frac{\partial \pi}{\partial a}\right)_T . \qquad \text{(S102)}$$

To stably calculate the derivative on the right hand side of this equation from the experimental data, we fit a polynomial of order 9 to the measured isotherm and use the analytical derivative of the fitted polynomial. As fig. S4 shows, the fitted polynomial shows excellent agreement with the experimental data.

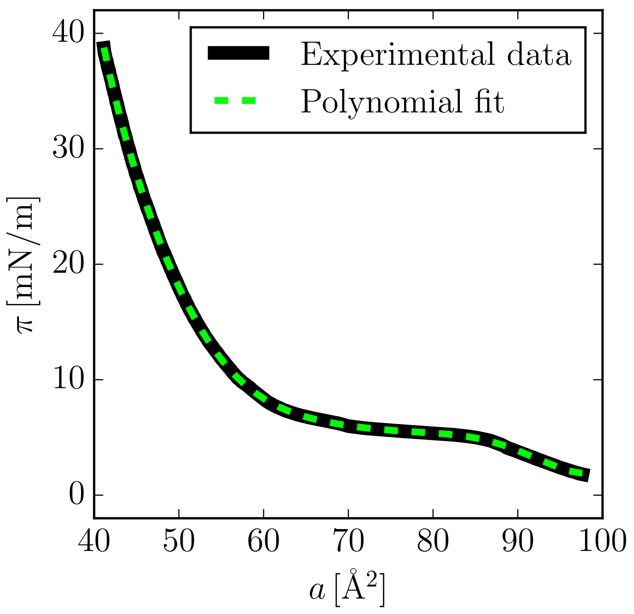


FIG. S4. **Experimentally measured pressure-area isotherm together with polynomial fit.** As explained in sect. S III, to calculate the elastic modulus $K_{2\mathrm{D}}$ for a DPPC monolayer on water, a polynomial (green dashed line) is fit to the experimental isotherm (black solid line).

## S IV. DISCUSSION OF THE LINEARIZATION ASSUMPTION FOR MOMENTUM CONSERVATION

The nonlinear fractional wave equation we use in the main text and derive in sect. S II is motivated by the dispersion relation of the Lucassen wave, which in turn is derived using the linearized Navier-Stokes equation, c.f. sect. S I. We therefore rely on the assumption, that the nonlinearity due to local changes in the elastic modulus $K_{2\mathrm{D}}$ is relevant, while the convective derivative term $(\vec{v}\cdot\vec{\nabla})\vec{v}$ of the velocity field, which appears in the Navier-Stokes equation, is negligible. In this section, we want to underpin this assumption.

For this, we assume that the displacement field in the $\hat{e}_x$-direction at the interface, $u_x(x, z=0, t) \equiv U(x,t)$, varies on a characteristic length scale $L$, and on a characteristic time scale $T$.

We first estimate the linearization condition for the Navier-Stokes equation,

$$|\partial_t^2 U| \gg |(\partial_t U)\partial_x(\partial_t U)|, \qquad \text{(S103)}$$

to be

$$\frac{|U|}{T^2} \gg \frac{|U|^2}{T^2 L}, \qquad \text{(S104)}$$

$$\Leftrightarrow \quad 1 \gg \frac{|U|}{L}. \qquad \text{(S105)}$$

To estimate when nonlinear effects due to local changes in the elastic modulus become important, we consider eq. (22) from the main text,

$$K_{2\mathrm{D}} = K_{2\mathrm{D}}^{(0)} + K_{2\mathrm{D}}^{(2)}\left(\bar{a} + \bar{a}\partial_x U(x,t) - a_0\right)^2 , \qquad \text{(S106)}$$

which gives the local elastic modulus as a function of the surface displacement field $U$. According to eq. (23) from the main text, nonlinear effects are negligible as long as the term linear in $U$ in eq. (S106) is small compared to the term independent of $U$ in eq. (S106), i.e. as long as

$$\left|2\bar{a}^2 K_{2\mathrm{D}}^{(2)}(1 - a_0/\bar{a})\partial_x U\right| \ll \left|K_{2\mathrm{D}}^{(0)} + \bar{a}^2 K_{2\mathrm{D}}^{(2)}(1 - a_0/\bar{a})^2\right|, \qquad \text{(S107)}$$

which leads to the estimate

$$\frac{|U|}{L} \ll \left| \frac{K_{2D}^{(0)} + \bar{a}^2 K_{2D}^{(2)} (1 - a_0/\bar{a})^2}{2\bar{a}^2 K_{2D}^{(2)} (1 - a_0/\bar{a})} \right| . \tag{S108}$$

Comparing this inequality to eq. (S105), we see that which nonlinearity becomes important first as the displacement $U$ increases depends on the value of

$$f(\bar{a}) := \left| \frac{K_{2D}^{(0)} + \bar{a}^2 K_{2D}^{(2)} (1 - a_0/\bar{a})^2}{2\bar{a}^2 K_{2D}^{(2)} (1 - a_0/\bar{a})} \right| . \tag{S109}$$

We plot $f$ in fig. S5, and as can be seen, except for equilibrium areas $\bar{a}$ close to the minimum of the elastic modulus, $f$ is of the order of 0.1, so that inequality (S108) will be violated at amplitudes much lower than inequality (S105). We therefore expect the nonlinearity arising from changes in the elastic modulus to become relevant approximately one order of magnitude below the convective nonlinearity in the Navier-Stokes equation. Thus, our premise of including one nonlinearity but not the other, is reasonable.

Note furthermore that inequality (S105) is also the basis for neglecting the term $1/(1 + \partial_x U)$ in going from eq. (S98) to eq. (S99) in sect. S II, and furthermore the justification for neglecting quadratic terms in the strain tensor [16].

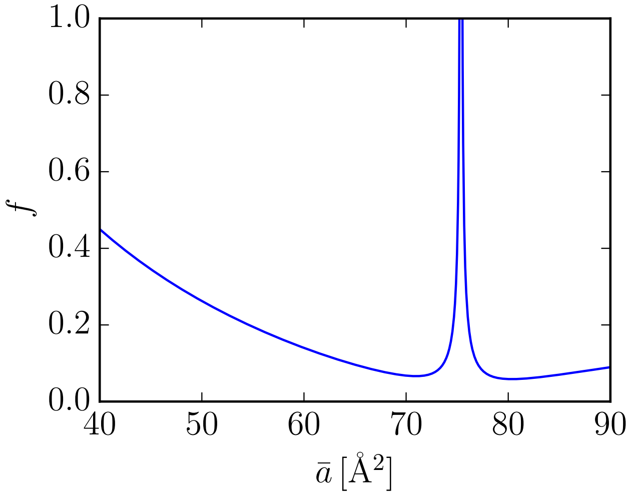


FIG. S5. **Comparison of relevance for nonlinear effects from convective derivative in the Navier-Stokes equation and area per lipid dependence of the elastic modulus** $K_{2D}$**.** The function $f$ as defined by eq. (S109) is plotted as a function of equilibrium area per lipid $\bar{a}$. For the other parameters appearing in $f$, the values from the main text are used, namely $K_{2D}^{(0)} = 2.55$ mN/m, $a_0 = 75.4\,\text{Å}^2$ and $K_{2D}^{(2)} = 0.12$ mN/(mÅ$^2$).

## S V. ISOTHERMAL VS. ADIABATIC ELASTIC MODULUS

Throughout this work, we use the isothermal elastic modulus for the elastic modulus $K_{2D}$ appearing in the Lucassen dispersion relation and the fractional wave equation. Whether this is appropriate, however, is a question of time scales: The isothermal elastic modulus is only appropriate if the compression and expansion of the interface during wave propagation is slow compared to the time scale of heat exchange with the bulk medium below, so that the temperature within the interface can be assumed to be constant. In the opposite limit, i.e. if the compression and expansion of the interface is so fast that there is no heat exchange during one oscillation, the adiabatic elastic modulus is the appropriate choice [17].

In this section we discuss whether the thermodynamics of the interface during wave propagation is isothermal or adiabatic. We do this by comparing the time scales of heat conduction within the bulk medium below the membrane to the time scale of the wave oscillation.

To estimate the time scale for heat conduction in the bulk medium, we consider the standard balance equation for the internal energy in the medium below the interface ($z < 0$), which in the absence of external forces reads

$$\rho \frac{\mathrm{d}e}{\mathrm{d}t} = \sigma_{ij} \partial_j v_i + \partial_i \left( \kappa \, \partial_i T \right) , \tag{S110}$$

where $\rho$ is the density, $e$ is the internal energy per unit mass, $\sigma$ is the stress tensor and $\kappa$ is the heat conduction coefficient. The first term on the right hand side of eq. (S110) models changes in internal energy due to viscous dissipation, while the second term on the right hand side models changes in the internal energy due to heat conduction.

Neglecting the first term (c.f. sect. S IV and note that the first term is quadratic in the velocity) and using $\mathrm{d}e/\mathrm{d}t \approx \partial e/\partial t = c_p \partial T/\partial t$ with $c_p$ the isobaric specific heat capacity (note that this is an approximation, as the pressure in the bulk medium is not strictly constant), we get

$$\rho c_p \frac{\partial T}{\partial t} = \partial_i \left( \kappa \, \partial_i T \right) , \tag{S111}$$

so that we obtain the relation

$$\tau_T \sim \frac{\rho c_p L^2}{\kappa} , \tag{S112}$$

for the time scale $\tau_T$ in which temperature equilibrates over a length scale $L$. For water, the parameters are $c_p = 4$ kJ/(kg · K), $\rho = 10^3$ kg/m$^3$, $\kappa = 0.6$ J/(m · s · K) [9]. We will now use the relation eq. (S112) to compare the time scale of heat conduction in the fluid below the surface to the time scale of the Lucassen wave that propagates along the surface. For this, we use the dispersion relation

$$k(\omega) = e^{i\pi/8} \sqrt{\frac{\sqrt{\rho \eta \omega^3}}{K_{2D}}} \tag{S113}$$

of the Lucassen wave, derived in sect. S I, c.f. eq. (S58).

- First, we consider heat conduction parallel to the interface: The frequency dependent wavelength of the Lucassen wave sets the length scale, and is given by

$$L = \frac{1}{\mathrm{Re}\,[k(\omega)]} = \frac{\sqrt{K_{2\mathrm{D}}}}{\cos(\pi/8)(\rho\eta\omega^3)^{1/4}}. \tag{S114}$$

Thus, the time scale for "parallel" thermal equilibration of the water below the surface is given by

$$\tau_T \sim \frac{\rho c_p K_{2\mathrm{D}}}{\kappa \cos^2(\pi/8)} \sqrt{\frac{\rho}{\eta\omega^3}}. \tag{S115}$$

This time scale is of the order of the time scale of oscillations, $\tau = 1/\omega$, if

$$\tau \sim \tau_T \tag{S116}$$

$$\iff \quad \omega \sim \frac{c_p^2 K_{2\mathrm{D}}^2 \rho}{\kappa^2 \eta \cos^4(\pi/8)} \approx 6 \cdot 10^9\ \frac{1}{\mathrm{s}}, \tag{S117}$$

where we use $K_{2\mathrm{D}} \approx 10^{-2}$ N/m as an order-of-magnitude estimate for the elastic modulus. For smaller frequencies, the time scale of thermal diffusion parallel to the surface is larger than the time scale of oscillations ($\tau < \tau_T$, adiabatic), while for larger frequencies, the time scale of thermal diffusion parallel to the surface is smaller than the time scale of oscillations ($\tau > \tau_T$, isothermal).

- Second, we consider heat conduction perpendicular to the interface: For this, the relevant length scale is the decay length of the wave away from the interface (i.e. the distance of the oscillating surface to the "bulk water reservoir"), which for the Lucassen wave is given by

$$L = \frac{1}{\mathrm{Re}(\lambda_t^{-1})} = \sqrt{\frac{2\eta}{\rho\omega}}, \tag{S118}$$

c.f. eq. (S47) (and note that the factorization condition eq. (S46) holds for a Lucassen wave on water, as discussed in sect. S I E). Comparing the resulting time scale for heat conduction with the time scale of oscillations, $\tau = 1/\omega$, we obtain

$$\tau \sim \tau_T \tag{S119}$$

$$\iff \quad 1 \sim \frac{c_p \eta}{\kappa} \approx 13. \tag{S120}$$

Since both time scales have the same frequency dependence, the crossover is independent of $\omega$, so that it only depends on the system parameters. Since eq. (S112) is only a rough estimate, we conclude from eq. (S120) that there is no clear separation of the time scales $\tau$, $\tau_T$.

From these order-of-magnitude estimates, we conclude that for water, heat conduction parallel to the surface can be ignored, while heat conduction away from the surface happens on a time scale comparable to the wave oscillations. Thus, the elastic modulus $K_{2\mathrm{D}}$ appropriate for the Lucassen wave is neither isothermal nor adiabatic, but somewhere in between.

For simplicity and because it is experimentally readily accessible, we chose the isothermal elastic modulus in the main text, but in view of the estimates performed in this section, this is clearly an approximation.

## S VI. ANALYTICAL SOLUTION OF LINEAR THEORY

In this section we consider the linearized fractional wave equation, i.e. eq. (17) of the main text with $\rho_{2\mathrm{D}} = 0$,

$$K_{2\mathrm{D}} \frac{\partial^2 U}{\partial x^2} = \sqrt{\rho\eta} \frac{\partial^{3/2} U}{\partial t^{3/2}}. \tag{S121}$$

This is a fractional wave equation, i.e. a wave equation where the second order time derivative has been replaced with a fractional derivative $\alpha \in (1, 2]$, which in our case is $\alpha = 3/2$. The fundamental solution (also called propagator or Green function) to the fractional wave equation was first derived by Schneider and Wyss in the 80s [18], the derivation was later simplified by Mainardi [19, 20].

We follow ref. [20] to discuss the signaling problem for eq. (S121), which is the appropriate boundary value problem for the experimental setup we want to model. In ref. [20], the signaling problem is defined as the following the boundary value problem:

$$\frac{\partial^{2\nu} U}{\partial t^{2\nu}} = D_0 \frac{\partial^2 U}{\partial x^2} \quad \forall (x, t) \in [0, \infty) \times [0, \infty), \tag{S122}$$

$$U(x, 0^+) = 0 \qquad \forall x \in (0, \infty), \tag{S123}$$

$$U(0^+, t) = U_0(t) \qquad \forall t \in (0, \infty), \tag{S124}$$

$$U(\infty, t) = 0 \qquad \forall t \in (0, \infty), \tag{S125}$$

where $U_0(t)$ is a given function that models a time dependent excitation at the boundary $x = 0$. In view of eq. (S121), we will later set $D_0 = K_{2\mathrm{D}}/\sqrt{\rho\eta}$ and will be interested in the case $\nu = 3/4$. For the sake of generality, we quote here the results for arbitrary $\nu \in (0, 1)$. For the particular choice $U_0(t) = \delta(t)$, the solution is called the propagator and written $\mathcal{G}_s(x, t; \nu)$. Given any other function $U_0(t)$, the respective solution to the signaling problem is then given as linear superposition of fundamental solutions, by

$$U(x, t; \nu) = \int_{0^-}^{t^+} \mathcal{G}_s(x, t - \tau; \nu) U_0(\tau)\ \mathrm{d}\tau, \tag{S126}$$

see eq. (6.9b) of ref. [20]. In chapter 6 of ref. [20], it is shown that $\mathcal{G}_s$ is given by

$$\mathcal{G}_s(x, t; \nu) = \frac{\nu x}{t^{1+\nu}\sqrt{D_0}} M_\nu \left( \frac{x}{t^\nu \sqrt{D_0}} \right), \tag{S127}$$

where $M_\nu(z)$ is given by the power series

$$M_\nu(z) = \frac{1}{\pi}\sum_{n=1}^{\infty}\frac{(-z)^{n-1}}{(n-1)!}\Gamma(\nu n)\sin(\pi\nu n), \tag{S128}$$

which converges for all $z \in \mathbb{C}$.

Since, as $|z|$ increases, the series (S128) converges more and more slowly, ref. [20] gives the asymptotic formula

$$M_\nu(\xi/\nu) \sim A_\nu(\xi/\nu) := \frac{\xi^{(\nu-1/2)/(1-\nu)}}{\sqrt{2\pi(1-\nu)}} \times \exp\left[-\frac{1-\nu}{\nu}\xi^{1/(1-\nu)}\right], \tag{S129}$$

valid for $|\xi/\nu| \to \infty$. Since for us, the case $\nu = 3/4$ with real $z$ is most relevant, we plot the function $M_{3/4}(x)$ as calculated from the power series eq. (S128), together with the asymptotic formula $A_{3/4}(x)$, eq. (S129), in fig. S6. As stopping criterion for the numerical summation of the power series (S128), we use that the relative change of the absolute value of the partial sum should be smaller than $10^{-8}$, i.e. we sum in eq. (S128) until term number

$$N := \inf\left\{ K \in \mathbb{N} \;\middle|\; \frac{|z|^K\Gamma(3/4\cdot(K+1))/K!}{\pi|M^K_{3/4}(z)|} < 10^{-8} \right\} + 1, \tag{S130}$$

where $M^K_{3/4}(z)$ is the partial sum of the power series in eq. (S128) (for $\nu = 3/4$) up to the $K$-th term. The calculations are performed at 500 digit floating point precision using the python module mpmath [21]. From fig. S6 we conclude that the asymptotic formula approximates $M_{3/4}(x)$ well for $x > 4$, meaning that the relative error $|A_{3/4}(x) - M_{3/4}(x)|/|M_{3/4}(x)| < 0.1\%$ for $x > 4$. For all subsequent evaluations of $M_{3/4}$(x) we therefore proceed as follows:

- Using eq. (S128), we pre-calculate a table of values for $M_{3/4}$ on the grid

$$\left\{i\cdot\Delta x \mid \Delta x = 0.001,\ i \in \{0, 1, ..., 4\cdot 10^3\}\right\}, \tag{S131}$$

  and then use linear interpolation on that dataset to evaluate $M_{3/4}(x)$ for $0 \le x \le 4$.

- For $x > 4$, we use the asymptotic formula (S129).

## S VII. NUMERICAL ALGORITHM FOR SOLVING THE NONLINEAR FRACTIONAL WAVE EQUATION

### A. Introduction

In this section, we present and validate a numerical scheme for solving the nonlinear fractional wave equation, eq. (23) from the main text. More specifically, we

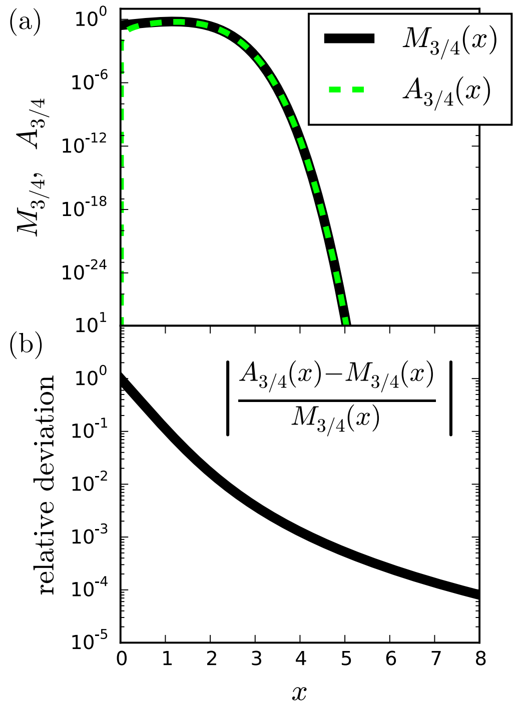


FIG. S6. **(a):** The functions $M_{3/4}$, $A_{3/4}$ as defined in eqs. (S128), (S129); **(b):** The relative deviation $|A_{3/4} - M_{3/4}|/|M_{3/4}|$ of the asymptotic expansion $A_{3/4}$ of $M_{3/4}$.

discuss a nonlinear version of the signaling problem from sect. S VI, i.e. we consider the boundary value problem

$$\frac{\partial^{2\nu}U}{\partial t^{2\nu}} = D(\partial_x U)\frac{\partial^2 U}{\partial x^2} \qquad \forall (x,t) \in [0,L]\times[0,\infty), \tag{S132}$$

$$U(x,0^+) = (\partial_t U)(x,0^+) = 0 \qquad \forall x \in (0,L), \tag{S133}$$

$$U(0^+,t) = U_0(t) \qquad \forall t \in (0,\infty), \tag{S134}$$

$$u(L^-,t) = U_L(t) \qquad \forall t \in (0,\infty), \tag{S135}$$

where $U_0$, $U_L$ are given functions that model imposed displacements at the boundaries of a system of length $L$. While $U_0$ will model a mechanical excitation at $x = 0$, $U_L$ will be set to zero later to model a rigid wall at $x = L$. $D$ is a function that depends on $\partial_x U$ locally, i.e. $D(\partial_x U)(x) = D(\partial_x U(x))$, and if it is non-constant, the eq. (S132) is nonlinear. While we state the algorithm for an arbitrary function $D$, in view of eq. (23) from the main text we will later be interested in the case where $D$ is of the form

$$D(\partial_x U) = \frac{K^{(0)}_{2\mathrm{D}} + K^{(2)}_{2\mathrm{D}}\left(\bar{a} + \bar{a}\partial_x U - a_0\right)^2}{\sqrt{\rho\eta}}. \tag{S136}$$

For the sake of generality, we also state the algorithm for arbitrary fractional derivative $\nu \in (1/2, 1)$, although we will later be interested in the case $\nu = 3/4$.

Before starting, we remark that, apart from the nonlinearity, the only difference between eqs. (S122-S125) and

eqs. (S132-S135) is that, while in the former the spatial domain is $[0,\infty)$, we in this section assume a bounded domain $[0,L]$. The reason for this is that a numerical solution can only be calculated on a finite domain, and that there seems to be no satisfactory way to implement free boundary conditions numerically. Our approach therefore is to calculate the numerical solution on a finite domain $[0,L]$ with boundary condition $U_L(t)\equiv 0$, and to choose $L$ large enough so that for a subinterval $[0,l]$ with $l \ll L$ we can effectively speak of free boundary conditions at $x=l$. We discuss an appropriate choice for $L$ for our system in sect. S VIII E, by comparing numerical solutions for the linear theory to the analytical solution from sect. S VI.

### B. Methods

To solve the boundary value problem given by eqs. (S132-S135) numerically, we discretize the equation in time and space and use the backward Euler-method to calculate the time evolution of the displacement field.

For the temporal discretization we follow Li et. al. [22], where a numerical scheme for a class of nonlinear fractional wave equations (which does not include eq. (S132)) is presented. They discretize time with a timestep $\Delta t$, and only consider $U(x,t)$ at times

$$t_j := j\cdot\Delta t \qquad j\in\mathbb{N}. \tag{S137}$$

To discretize the fractional derivative [20],

$$\frac{\partial^{2\nu}U}{\partial t^{2\nu}}(x,t)=\frac{1}{\Gamma(1-2\nu)}\int_0^t\left[\frac{\partial^2}{\partial\tau^2}U(x,\tau)\right]\frac{1}{(t-\tau)^{2\nu-1}}\,\mathrm{d}\tau, \tag{S138}$$

with $\Gamma$ is the Gamma function, they approximate the second derivative of $U(x,t)$ using the center difference scheme, and take this second derivative to be constant in each interval $(t_j,t_{j+1})$. Then, after writing the integral on the RHS of eq. (S138) as a sum over integrals over all the subintervals $(t_j,t_{j+1})$, these can be evaluated to obtain the approximate formula

$$\frac{\partial^{2\nu}U}{\partial t^{2\nu}}(x,t_{m+1})=\frac{(\Delta t)^{-\alpha}}{\Gamma(3-\alpha)}\left(-\omega_0U(x,t_{m+1})-\sum_{j=-1}^{m}b_j^mU(x,t_m)\right), \tag{S139}$$

where the scalars $b_j^m$ are defined by

$$b_j^m:=\begin{cases}-\omega_m & j=-1,\\ 2\omega_m-\omega_{m-1} & j=0,\\ -\omega_{m-j+1}+2\omega_{m-j}-\omega_{m-j-1} & 1\le j\le m-1,\\ -\omega_1+2\omega_0 & j=m,\end{cases} \tag{S140}$$

and

$$\omega_j:=(j+1)^{2(1-\nu)}-j^{2(1-\nu)}. \tag{S141}$$

The initial conditions enter eq. (S139) via $U(x,0)$ and

$$U(x,t_{-1}):=U(x,0)-\Delta t(\partial_tU)(x,0). \tag{S142}$$

In our particular situation, both $U(x,t)$ and $U(x,t_{-1})$ are zero, c.f. eq. (S133).

To discretize space, we divide the interval $[0,L]$ into $N+1$ subintervals of equal length $\Delta x := L/(N+1)$. The $N+2$ boundary points of these subintervals are then given by the positions

$$x_j := j\cdot\Delta x \qquad j\in\{0,...,N+1\}. \tag{S143}$$

We discretize the second order spatial derivative in eq. (S132) using the center difference scheme, i.e. we approximate

$$\frac{\partial^2U}{\partial x^2}(x_n,t)=\frac{U(x_{n+1},t)-2U(x_n,t)+U(x_{n-1},t)}{\Delta x^2}. \tag{S144}$$

Note that $U(x_0,t)$, $U(x_{N+1},t)$ are given by the spatial boundary conditions,

$$U(x_0,t)\equiv U_0(t), \tag{S145}$$
$$U(x_{N+1},t)\equiv U_L(t). \tag{S146}$$

Since we want to calculate $U(x,t)$ on the grid $(x_n,t_m)$, we introduce the notation

$$U_n^m := U(x_n,t_m). \tag{S147}$$

With this notation, and using eqs. (S139), (S144), we obtain a discretized version of eq. (S132), given by

$$\left(\omega_0\mathbb{I}_{N,N+2}+\lambda W\left(\vec{U}^{m+1}\right)\right)\vec{U}^{m+1}=\sum_{j=-1}^{n}b_j^n\vec{U}^m, \tag{S148}$$

where

$$\lambda=\frac{\Gamma(3-2\nu)(\Delta t)^{2\nu}}{\Delta x^2}, \tag{S149}$$

the $N+1$ dimensional vector $\vec{U}^k$ is given by

$$\vec{U}^k:=\begin{pmatrix}U_0^k\\ U_1^k\\ \vdots\\ U_N^k\\ U_{N+1}^k\end{pmatrix} \qquad k\in\mathbb{N}, \tag{S150}$$

and the two $N\times(N+2)$ matrices $\mathbb{I}_{N,N+2}$, $W$ are given by

$$\mathbb{I}_{N,N+2} := \begin{pmatrix} 0 & 1 & 0 & 0 & & \cdots & 0 & 0 \\ 0 & 0 & 1 & 0 & 0 & & \vdots & 0 \\ \vdots & 0 & 0 & 1 & 0 & \ddots & \vdots & \vdots \\ \vdots & & \ddots & 0 & \ddots & \ddots & 0 & \vdots \\ \vdots & & & \ddots & \ddots & \ddots & 0 & 0 \\ 0 & \cdots & \cdots & \cdots & 0 & 0 & 1 & 0 \end{pmatrix} \in \mathbb{R}^{N\times(N+2)}, \tag{S151}$$

$$W(\vec{U}^m) := \begin{pmatrix} -W_1(\vec{U}^m) & 2W_1(\vec{U}^m) & -W_1(\vec{U}^m) & 0 & & \cdots & 0 & 0 \\ 0 & -W_2(\vec{U}^m) & 2W_2(\vec{U}^m) & -W_2(\vec{U}^m) & 0 & & \vdots & 0 \\ \vdots & 0 & -W_3(\vec{U}^m) & 2W_3(\vec{U}^m) & -W_3(\vec{U}^m) & \ddots & \vdots & \vdots \\ \vdots & & \ddots & -W_4 & \ddots & \ddots & 0 & \vdots \\ \vdots & & & \ddots & \ddots & \ddots & -W_{N-1}(\vec{U}^m) & 0 \\ 0 & \cdots & \cdots & \cdots & 0 & W_N(\vec{U}^m) & 2W_N(\vec{U}^m) & W_N(\vec{U}^m) \end{pmatrix} \in \mathbb{R}^{N\times(N+2)}, \tag{S152}$$

with

$$W_i(\vec{U}^m) = D\left(\frac{U_{i+1}^m - U_{i-1}^m}{2\Delta x}\right), \tag{S153}$$

where we used the symmetric approximation $\partial_x U(x_i, t_m) = (U_{i+1}^m - U_{i-1}^m)/(2\Delta x)$ for the derivative in the argument of $D$.

Note that while the vector $\vec{U}^k$ has $N+2$ elements, c.f. eq. (S150), at every timestep only $N$ of them are unknown because $U_0^k$, $U_{N+1}^k$ are fixed by the spatial boundary conditions, c.f. eqs. (S145), (S146). The discretized equation (S148) is an equation for the $N$ remaining components of $\vec{U}^k$ at every timestep.

### C. Special case: Linear theory

If we assume $D$ to be constant, i.e.

$$D(\partial_x U) \equiv D_0 \equiv const. \in (0, \infty), \tag{S154}$$

the matrix $W\left(\vec{U}^{m+1}\right)$ becomes independent of $\vec{U}^{m+1}$, c.f. eqs. (S152), (S153). It is then given by

$$W = D_0 \begin{pmatrix} -1 & 2 & -1 & 0 & & \cdots & & 0 & 0 \\ 0 & -1 & 2 & -1 & 0 & & & & \\ & 0 & -1 & 2 & -1 & \ddots & & \vdots & \vdots \\ \vdots & & \ddots & -1 & \ddots & \ddots & \ddots & & \vdots \\ \vdots & \vdots & & \ddots & \ddots & \ddots & -1 & 0 & \\ & & & & 0 & -1 & 2 & -1 & 0 \\ 0 & 0 & & \cdots & & 0 & -1 & 2 & -1 \end{pmatrix}, \tag{S155}$$

as can easily be verified by looking at the definition of the matrix elements, eq. (S153). Thus, the matrix eq. (S148) becomes linear and is given by

$$\left(\omega_0 \mathbb{I}_{N,N+2} + \lambda W\right) \vec{U}^{m+1} = \sum_{j=-1}^{n} b_j^n \vec{U}^m. \tag{S156}$$

## S VIII. LINEAR THEORY: COMPARISON OF ANALYTICAL AND NUMERICAL RESULTS

### A. Introduction

To validate the numerical algorithm from sect. S VII, we consider the linearized fractional wave equation,

i.e. the situation where $\nu = 3/4$ and

$$D_0 \equiv \frac{K_{2D}}{\sqrt{\rho\eta}} \equiv const., \tag{S157}$$

with $K_{2D}$ constant, c.f. eqs. (S136), (S154). For water,

$$\rho = 10^3 \text{ kg/m}^3, \tag{S158}$$
$$\eta = 10^{-3} \text{ Pa} \cdot \text{s}. \tag{S159}$$

In this section, we compare the analytical solution of the signaling problem, defined by eqs. (S122-S125), to the numerical solution of eqs. (S132-S135).

Note that, in the linear case, the only difference between the two boundary value problems is the right boundary: In the analytical solution, the spatial domain is $[0, \infty)$ with spatial boundary conditions $U(0,t) = U_0(t)$, $U(\infty, t) = 0$, with $U_0$ a given function, c.f. eqs. (S124), (S125). In the numerical scheme, the spatial domain is the bounded interval $[0, L]$ with spatial boundary conditions $U(0,t) = U_0(t)$, $U(L,t) = U_L(t)$, with $U_0$, $U_L$ given functions, c.f. eqs. (S134), (S135).

Although every experimental system is of finite size, it is usually chosen large enough so that boundary effects from the walls are not relevant, i.e. we are actually interested in the solution on an infinite spatial domain, as in the analytical solution. However, we expect that if we choose the right boundary condition in the numerical approach to be zero identically, $U_L(t) \equiv 0$, and we use an interval $[0, L]$ so large that, during the simulation time $T$, a field $U$ excited at the left boundary does not reach the right boundary (so that there is no reflection), and only consider the values of $U(x,t)$ for $x \in (0, l)$ with $l \ll L$ (i.e. sufficiently far away from the rigid wall at $x = L$), then we expect the numerical scheme to yield a solution comparable to the analytical one from sect. S VI.

## B. Parameters

Throughout this section, we use the parameters

$$L = 30 \text{ mm}, \tag{S160}$$
$$\Delta x = 0.1 \text{ mm}, \tag{S161}$$
$$\Delta t = 0.01 \text{ ms} \tag{S162}$$

for numerical solutions, while analytical solutions are directly evaluated on a lattice with the same spacings $\Delta x$, $\Delta t$.

The right boundary condition is set to zero in all numerical calculations, $U_L(t) \equiv 0$, for the left boundary condition we use a normalized discretized delta peak, i.e.

$$U_0^j \overset{(S145)}{=} U_0(j \cdot \Delta t) := \delta_{j,1} \frac{1}{\Delta t}. \tag{S163}$$

Accordingly, the analytical solution is always calculated using a delta peak initial condition at $x = 0$, i.e. using the propagator $\mathcal{G}_s(x, t; \nu)$ from sect. S VI.

We only consider the numerical solution for $x \leq 10$ mm $=: l$, so that $l/L = 1/3$, and up to times $T = 100$ ms.

In the following sections, we validate our choices for $L$, $l$, $T$, as well as for the discretization parameters $\Delta x$, $\Delta t$, by comparing numerical and analytical solutions.

## C. Position and time dependence of solutions at fixed $K_{2D}$

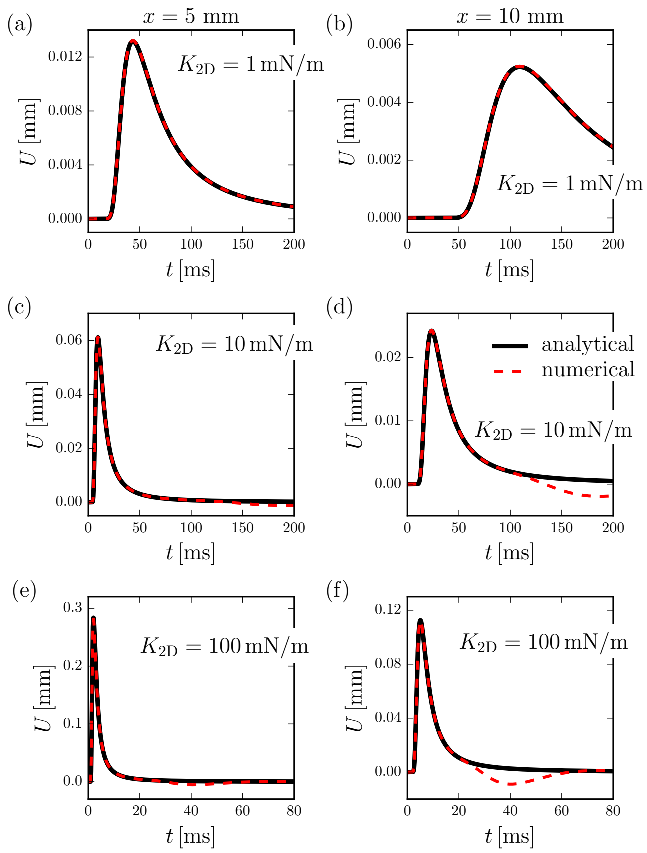


FIG. S7. **Displacement fields as calculated from the analytical and numerical solution to the linear fractional wave equation.** The parameters given in section S VIII B are used to calculate both the analytical and the numerical solution for elastic moduli $K_{2D} = 1$, 10, 100 mN/m. The respective solutions $U(x,t)$ are shown here as a function of time for $x = 5$ mm (left column) and $x = 10$ mm (right column).

Using the parameters from sect. S VIII B, we first compare numerical and analytical solutions for

$$K_{2D} \in \{1, \ 10, \ 100\} \text{ mN/m}. \tag{S164}$$

- Figure S7 shows the displacement fields at $x = 5$ mm and $x = 10$ mm as a function of time. Although there are deviations when the displacement

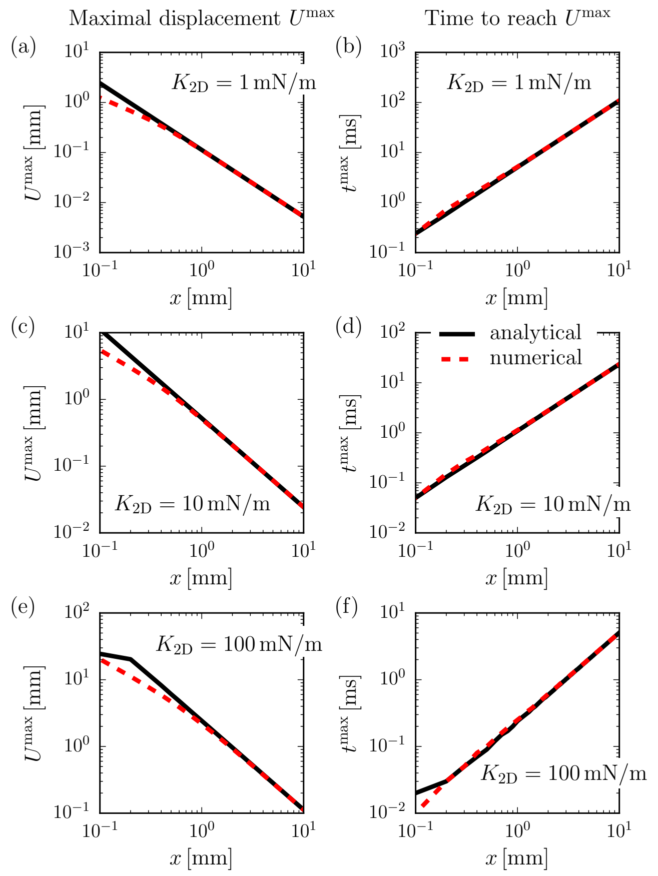


FIG. S8. **Maximal displacement and time needed until maximal displacement occurs as calculated from analytical and numerical solution of the linear fractional wave equation.** The parameters given in section S VIII B are used to calculate both the analytical and the numerical solution for elastic moduli $K_{2D} = 1$, 10, 100 mN/m. Using the respective solutions and eqs. (S166), (S166), the maximal displacement as a function of position and the time elapsed until this displacement occurs are calculated and shown here as functions of position $x$.

field has almost decayed (subplot (d) at $t = 150$-200 ms and subplot (f) around $t = 40$ ms), overall the displacement fields of numerical and analytical solutions agree very well.

- Figure S8 shows both the maximal displacement,

$$U^{\max}(x) := \max_t \{\, U(x,t) \,\}\,, \tag{S165}$$

and the time elapsed until this maximal displacement occurs,

$$t^{\max}(x) := \min_t \{\, U(x,t) = U^{\max}(x) \,\}\,, \tag{S166}$$

as a function of $x$, the distance from the left boundary. There are some deviations between numerical and analytical results close to the delta peak initial condition, namely for $x \lesssim 0.3$ mm, but for $x \gtrsim 1$ mm the solutions agree very well.

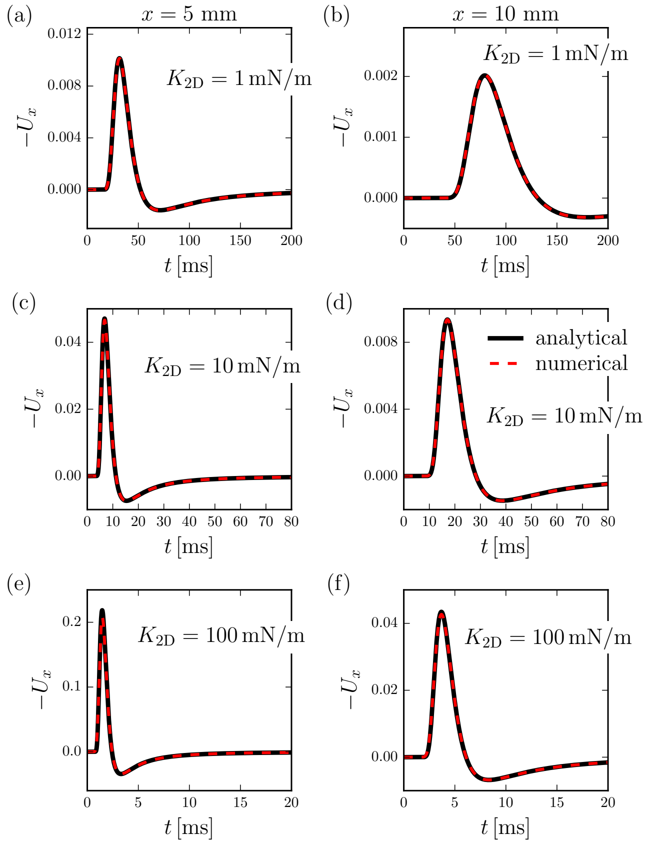


FIG. S9. **Compression fields as function of time as calculated from analytical and numerical solution of the linear fractional wave equation.** The parameters given in section S VIII B are used to calculate both the analytical and the numerical solution for elastic moduli $K_{2D} = 1$, 10, 100 mN/m. Using the respective solutions and eq. (S167), the compression field $-\partial_x U$ is calculated and shown here as a function of time for $x = 5$ mm (left column) and $x = 10$ mm (right column).

- Figure S9 shows the compresson fields, defined as

$$-\,U_x(x,t) = -\frac{\partial U}{\partial x}(x,t), \tag{S167}$$

calculated from the numerical solutions shown in fig. S7. Agreement between numerical and analytical solutions is excellent here. Note that the times $t$ at which deviations occured in fig. S7 are not shown here for better visibility of the main peaks (at $t = 20$ ms in subplot (d) and $t = 4$ ms in subplot (f)). However, since the numerical and analytical curves in fig. S7 have comparable slopes in the region where they deviate, the compression fields look quite similar even for the times where the displacement fields deviate.

- Figure S10 shows both the extremal values of com-

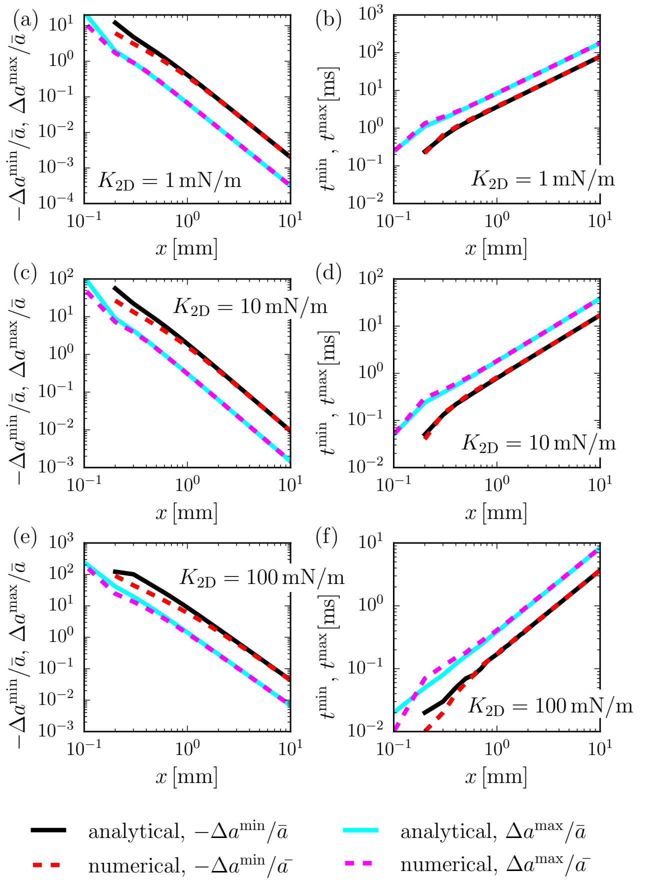


FIG. S10. **Extremal compression and expansion and time to reach these** as calculated from the analytical and numerical solution to the fractional wave equation. The parameters given in section S VIII B are used to calculate both the analytical and the numerical solution for elastic moduli $K_{2D} = 1$, 10, 100 mN/m. Using the respective solutions and eqs. (S168-S171), maximal compression $-\Delta a^{\min}/\bar{a}$ and maximal expansion $\Delta a^{\max}/\bar{a}$, as well as the time elapsed until these occur are calculated and shown here as functions of position $x$.

pression and expansion,

$$(-\Delta a^{\min}/\bar{a})(x) := \min_t \{\ \partial_x U(x,t)\ \}\,, \tag{S168}$$

$$(\Delta a^{\max}/\bar{a})(x) := \max_t \{\ \partial_x U(x,t)\ \}\,, \tag{S169}$$

and the time until these extremal values occur,

$$t^{\min}(x) := \min_t \left\{\ -\partial_x U(x,t) = (-\Delta a^{\min}/\bar{a})(x)\ \right\}, \tag{S170}$$

$$t^{\max}(x) := \min_t \{\ \partial_x U(x,t) = (\Delta a^{\max}/\bar{a})(x)\ \}\,, \tag{S171}$$

as a function of $x$. Close to the left boundary, there are deviations between numerical and analytical predictions, but for $x \gtrsim 1$ mm, they agree very well.

In summary, except for small distances $x \lesssim 1$ mm from the left boundary condition that are comparable to the spatial discretization $\Delta x = 0.1$ mm, the numerical and analytical results agree very well, validating both our numerical algorithm and our parameter choices for $L$, $\Delta x$, $\Delta t$.

### D. Elastic modulus depedence of compression and wave velocity at fixed position $x$

As a further check of consistency between numerical and analytical solution, we calculate the solutions for elastic moduli in the range

$$10^{-1} \leq \frac{K_{2D}}{\mathrm{mN/m}} \leq 10^3, \tag{S172}$$

and subsequenctly calculate both the maximal compression/expansion, as defined in eqs. (S168), (S169), at distances $x = 1$, 5, 9 mm, as well as the compression wave velocities, defined as

$$c^{\min}(x) = \frac{x}{t^{\min}(x)}, \tag{S173}$$

$$c^{\max}(x) = \frac{x}{t^{\max}(x)}, \tag{S174}$$

where $t^{\min}$, $t^{\max}$ are the times elapsed until the extremal compression occures, c.f. eqs. (S170), (S171). The results are shown in fig. S11. Except for the smallest distance $x = 1$ mm at small elastic moduli $K_{2D} \lesssim 1\,\mathrm{mN/m}$, numerical and analytical results agree very well.

### E. Conclusion

Based on the comparison between numerical and analytical solution carried out in sects. S VIII C, S VIII D, we conclude that our numerical algorithm works reliably and that our choice of parameters, $L = 30$ mm, $\Delta x = 0.1$ mm, $\Delta t = 0.01$ ms, is appropriate if we are interested in effects on the scales

$$1\ \mathrm{mm} \leq x \leq 10\ \mathrm{mm}, \tag{S175}$$

$$1\ \mathrm{ms} \leq t \leq 100\ \mathrm{ms}, \tag{S176}$$

and area moduli

$$0.1\ \mathrm{mN/m} \leq K \leq 100\ \mathrm{mN/m}. \tag{S177}$$

Thus, the value $l/L = 1/3$ is appropriate to emulate free boundary conditions at $x = 1$ cm for times $t \leq 100$ ms.

## S IX. OBTAINING THE NUMERICAL BOUNDARY CONDITION FROM EXPERIMENTAL DATA

To model the experimental excitation mechanism theoretically as a boundary condition, a DPPC monolayer

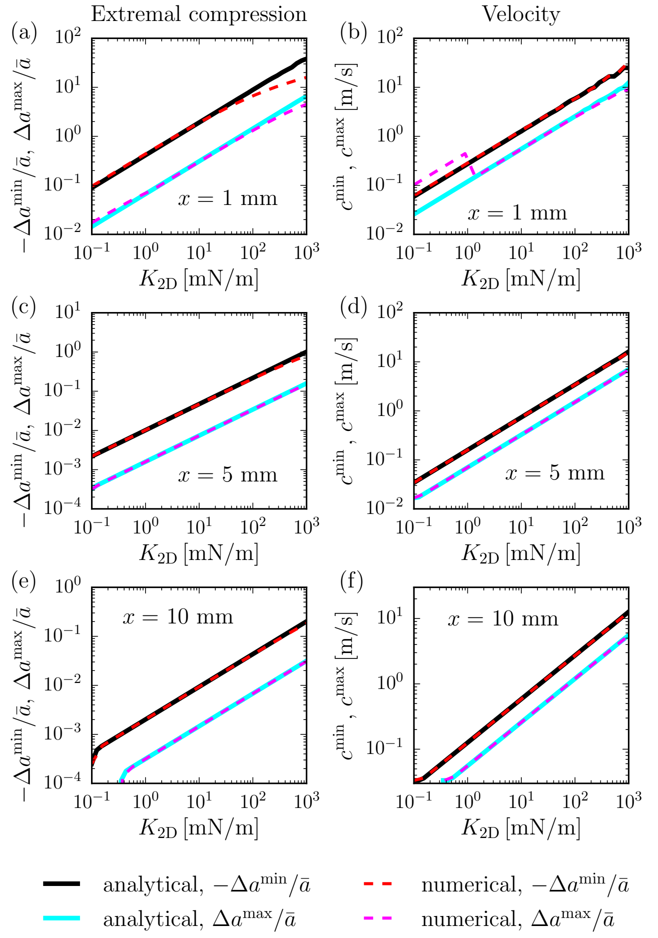


FIG. S11. **Dependence of analytical and numerical solution of the linear fractional wave equation on the elastic modulus.** The parameters given in section S VIII B are used to calculate both the analytical and the numerical solution for elastic moduli between $K_{2D} = 0.1$ mN/m and $K = 1000$ mN/m. Using these solutions and eq. (S167), first the compression field $-U_x$ is calculated. From the compression field, extremal values and propagation velocities for positions $x = 1, 5, 10$ mm are subsequently calculated using eqs. (S168), (S169), (S173), (S174). These extremal values and velocities are shown here as a function of the elastic modulus $K_{2D}$.

(without FRET marker) on water, at a surface pressure around 5 mN/m, is considered, details of the experimental setup are given in refs. [23–25]. The camera is focused on the razorblade, and the intensity as a function of time is recorded during an excitation. The result is shown in fig. S12 (a).

To model the excitation theoretically, a function of the form

$$U_0(t) = U_0^{\max} \cdot \begin{cases} \exp\left[-\left(t-t_1\right)^2/\tau^2\right] & t < t_1, \\ 1 & t_1 \le t \le t_2, \\ \exp\left[-\left(t-t_2\right)^2/\tau^2\right] & t_2 < t, \end{cases} \tag{S178}$$

is fitted to the first positive peak, see fig. S12 (b). The resulting fit parameters are $\tau^2 = 5.01$ ms$^2$, $t_1 = 18.39$ ms, $t_2 = 23.63$ ms. To save simulation time, we subtract 10 ms from both $t_1$ and $t_2$ in the main text.

## S X. ROBUSTNESS OF NONLINEAR NUMERICAL RESULTS WITH RESPECT TO VARYING ELASTIC MODULUS AND BOUNDARY CONDITION

To solve eq. (17) from the main text numerically, we need to input two functions:

- A function $K_{2D}(a)$ that describes how the elastic modulus changes as a function of area per lipid. In the main text, we use a quadratic fit to the experimentally obtained isothermal elastic modulus, c.f. sect. S III. The green dashed line in fig. S13 (a) shows a replot of the quadratic elastic modulus $K_{2D}$ we use in the main text, together with the elastic modulus obtained from experiment as described in sect. S III, and denoted in the following by $K_{2D}^{\exp}$.
- A function $U_0(t)$ for the boundary condition at $x = 0$. We discussed our choice for the main text in sect. S IX.

In this section we discuss the robustness of our nonlinear results with respect to varying both the elastic modulus function $K_{2D}$ and the boundary condition $U_0$. We do this by evaluating eq. (17) from the main text with $\rho_{2D}^{(0)} = 0$ for several different elastic modulus functions and boundary conditions, and calculating the maximal compression at $x = 8.4$ mm as well as the corresponding wave velocity, as defined by eqs. (29), (30) from the main text.

The main result from the following discussion is that the qualitative features of our nonlinear theory, a steep increase in observed compression accompanied by an increase in wave velocity, are roboust with respect to varying both the elastic modulus function $K_{2D}$ and the boundary condition $U_0$. However, the details, namely at which driving amplitude $U_0^{\max}$ the steep increase happens, how steep it is, and the wave velocity, depend on the exact form of both nonlinearity and boundary condition.

### A. Varying the elastic modulus

First, we consider three different elastic moduli:

- We consider a quadratic elastic modulus $K_{2D}^{I}$ that is fitted to $K_{2D}^{exp}$ (the experimentally obtained elastic modulus as discussed in sect. S III) in the region $a > a_{min}$, where $a_{min} \approx 80\,\text{Å}^2$ is the position of the minimum of $K_{2D}^{exp}$, with the additional constraint that the minimum of $K_{2D}^{I}$ be at the same point as the minimum of $K_{2D}^{exp}$, $(a_{min}, K_{2D}^{I}(a_{min})) = (a_{min}, K_{2D}^{exp}(a_{min}))$. $K_{2D}^{I}$ is shown in fig. S13 (b).

- For $K_{2D}^{II}$, we use the experimental $K_{2D}^{exp}$ directly and extend the elastic modulus as constant outside of the region where experimental data is available,

$$K_{2D}^{II}(a) := \begin{cases} K_{2D}^{exp}(a_L) & a < a_L, \\ K_{2D}^{exp}(a) & a_L < a < a_R, \\ K_{2D}^{exp}(a_R) & a_R < a, \end{cases} \tag{S179}$$

where $K_{2D}^{exp}$ is the experimental isothermal elastic modulus as discussed in sect. S III, $a_L = 45\,\text{Å}^2$ and $a_R = 90\,\text{Å}^2$. $K_{2D}^{II}$ is shown in fig. S13 (c).

- While $K_{2D}^{II}$ extrapolates beyond the experimental data in a very simple way, it is clearly unphysical: The elastic modulus is expected to diverge as the area per lipid $a$ decreases (at some point, of course the monolayer is expected to disintegrate if it gets more and more compressed), while it is expected to approach zero as the area per lipid increases. Therefore, we also consider

$$K_{2D}^{III}(a) := \begin{cases} K_{2D}^{III,L}(a) & a < a_L, \\ K_{2D}^{exp}(a) & a_L < a < a_R, \\ K_{2D}^{III,R}(a) & a_R < a, \end{cases} \tag{S180}$$

where again $K_{2D}^{exp}(a)$ is the experimental isothermal elastic modulus introduced in sect. S III, $K_{2D}^{III,L}$ is a second order polynomial and $K_{2D}^{III,R}(a) = a_1^R a^{-1} + a_2^R a^{-2}$. The polynomial $K_{2D}^{III,L}$ and the coefficients $a_1^R$, $a_2^R$ are chosen such that $K_{2D}^{III}$ and its first derivative are continuous at $a_L = 45\,\text{Å}^2$, $a_R = 90\,\text{Å}^2$. $K_{2D}^{III}$ is shown in fig. S13 (d).

Using the same boundary condition as we use in the main text, c.f. sect. S IX, and the initial area per lipid $\bar{a} = 88.4\,\text{Å}^2$, we evaluate eq. (17) from the main text with $\rho_{2D} = 0$ for the area moduli $K_{2D}^{I}$, $K_{2D}^{II}$, $K_{2D}^{III}$. Using eqs. (28-30) from the main text, we calculate maximal compression $-\Delta a^{min}/\bar{a}$ and wave speed $c$ at a distance $x = 8.4$ mm from the excitation source (which is at $x = 0$). The results, together with the corresponding results obtained from using the quadratic $K_{2D}$ from the main text, are shown fig. S14. As the figure shows, all elastic modulus functions yield qualitatively similar results. The most notable difference is that the threshold amplitude, i.e. the value of $U_0^{max}$ at which $-\Delta a^{min}/\bar{a}$ increases steeply, is sensitive to the detailed form of the elastic modulus function, see fig. S14 (c). Overall, we can conclude that the main features of our nonlinear results (a steep increase in observed compression accompanied by an increase in wave velocity) are robust w.r.t. varying the elastic modulus.

### B. Different boundary conditions

In sect. S IX, we fitted a function of the form

$$U(t) = U_0^{max} \cdot \begin{cases} \exp\left[-\left(t - t_1\right)^2/\tau^2\right] & t < t_1, \\ 1 & t_1 \le t \le t_2, \\ \exp\left[-\left(t - 2_1\right)^2/\tau^2\right] & t_2 < t \end{cases} \tag{S181}$$

to parts of the intensity time series recorded by a camera during excitation of the razor blade, to obtain the boundary condition we use the main text.

To better gauge the influence of the boundary condition on the results of the nonlinear theory, we consider several other boundary conditions in this section, namely:

- The full recorded intensity time series, c.f. sect. S IX, rescaled such that the maximal positive displacement is $U_0^{max}$.

- Smoothed rectangular functions eq. (S181) of different plateau width $\tau_p := t_2 - t_1$ and steepness $\tau$.

- Smoothed step functions, obtained by setting $t_2 = \infty$ in eq. (S181), for several values of $\tau$.

These boundary conditions are shown in figs. S15 (a) and S16, the corresponding parameter values are given in table I. For all these boundary conditions, we evaluate eq. (23) from the main text at the equilibrium area per lipid $\bar{a} = 88.4\,\text{Å}^2$. Using eqs. (28-30) from the main text, we subsequently calculate maximal compression $-\Delta a^{min}/\bar{a}$ and wave speed $c$ at a distance $x = 8.4$ mm from the excitation source (which is at $x = 0$).

In fig. S15 we show the numerical results for using the full recorded intensity profile as boundary condition. As subplots (c), (d) show, using the recorded intensity profile also yields a steep increase in compression accompagnied by an increase in wave speed. However, as subplot (b) shows, the driving amplitude $U_0^{max}$ at which the steep increase occures is decreased by factor of about 3.

In fig. S16 we show the smoothed rectangular functions and step functions considered, and in fig. S17 we show the corresponding results. As the figures show, all boundary conditions produce qualitatively similar results, in particular they all produce a steep increase in $-\Delta a^{min}/\bar{a}$ at a threshold driving amplitude that is accompanied by an increase in wave speed $c$. The exact position of this increase, however, depends on the details of the boundary condition, with the step function yielding a rather weak increase (as compared to the smoothed rectangular functions), compare figs. S17 (c), (f), (i) with fig. S17 (l). In

| Subplot of fig. S16 | $t_1$ [ms] | $t_2$ [ms] | $\tau^2$ [ms$^2$] |
|---|---|---|---|
| (c) | 18 | 19 | 0.1 |
| | 18 | 19 | 1 |
| | 18 | 19 | 5 |
| | 18 | 19 | 10 |
| (d) | 18 | 23 | 0.1 |
| | 18 | 23 | 1 |
| | 18 | 23 | 5 |
| | 18 | 23 | 10 |
| (e) | 18 | 28 | 0.1 |
| | 18 | 28 | 1 |
| | 18 | 28 | 5 |
| | 18 | 28 | 10 |
| (f) | 18 | $\infty$ | 0.1 |
| | 18 | $\infty$ | 1 |
| | 18 | $\infty$ | 5 |
| | 18 | $\infty$ | 10 |

TABLE I. Parameters for the boundary conditions considered in sect. S X B, c.f. eq. (S181) and figs. S16, S17.

summary, we can conclude that the main features of our nonlinear results (a steep increase in observed compression accompanied by an increase in wave velocity) are also robust w.r.t. to varying the boundary condition.


[1] J. Kappler and R. R. Netz, EPL (Europhysics Letters) **112**, 19002 (2015).
[2] D. J. Acheson, *Elementary Fluid Dynamics*, Oxford Applied Mathematics and Computing Science Series (Clarendon Press, 1990).
[3] P. A. Kralchevsky, J. C. Eriksson, and S. Ljunggren, Advances in Colloid and Interface Science **48**, 19 (1994).
[4] This is ([3],5.16), ([3],5.17), but with the membrane inertia and body force kept. Also in eq. ([3],5.16), the stress tensor of the medium above the membrane was neglected, which we included.
[5] L. Landau, E. Lifshitz, A. Kosevich, and L. Pitaevskiĭ, *Theory of Elasticity*, Course of theoretical physics (Butterworth-Heinemann, 1986).
[6] J. Lucassen, Trans. Faraday Soc. **64**, 2221 (1968).
[7] T. Chou, Journal of Fluid Mechanics **369**, 333 (1998).
[8] J. Lucassen and M. V. D. Tempel, Journal of Colloid and Interface Science **41**, 491 (1972).
[9] W. M. Haynes, *CRC Handbook of Chemistry and Physics, 95th Edition* (CRC Press, 2014) p. 2704.
[10] J. Krägel, J. B. Li, R. Miller, M. Bree, G. Kretzschmar, and H. Möhwald, Colloid and Polymer Science **274**, 1183 (1996).
[11] J. Griesbauer, S. Bössinger, A. Wixforth, and M. F. Schneider, Phys. Rev. Lett. **108**, 198103 (2012).
[12] E. P. Petrov, R. Petrosyan, and P. Schwille, Soft Matter **8**, 7552 (2012).
[13] E. P. Petrov and P. Schwille, Biophysical Journal **94**, L41 (2008).
[14] C.-H. Lee, W.-C. Lin, and J. Wang, Phys. Rev. E **64**, 020901 (2001).
[15] N. Delorme and A. Fery, Physical Review E **74**, 030901 (2006).
[16] J. Marsden and T. Hughes, *Mathematical Foundations of Elasticity*, Dover Civil and Mechanical Engineering Series (Dover, 1994).
[17] W. W. Van Osdol, R. L. Biltonen, and M. L. Johnson, Journal of Biochemical and Biophysical Methods **20**, 1 (1989).
[18] W. R. Schneider and W. Wyss, Journal of Mathematical Physics **30**, 134 (1989).
[19] F. Mainardi, Applied Mathematics Letters **9**, 23 (1996).
[20] F. Mainardi, *Fractional Calculus and Waves in Linear Viscoelasticity: An Introduction to Mathematical Models* (World Scientific, 2010) p. 368.
[21] F. Johansson *et al.*, *mpmath: a Python library for arbitrary-precision floating-point arithmetic (version 0.14)* (2010), `http://code.google.com/p/mpmath/`.
[22] C. Li, Z. Zhao, and Y. Chen, Comput. Math. Appl. **62**, 855 (2011).
[23] S. Shrivastava and M. F. Schneider, PLoS ONE **8**, 1 (2013).
[24] S. Shrivastava and M. F. Schneider, Journal of the Royal Society, Interface / the Royal Society **11**, 20140098 (2014).
[25] S. Shrivastava, K. H. Kang, and M. F. Schneider, Phys. Rev. E **91**, 012715 (2015).

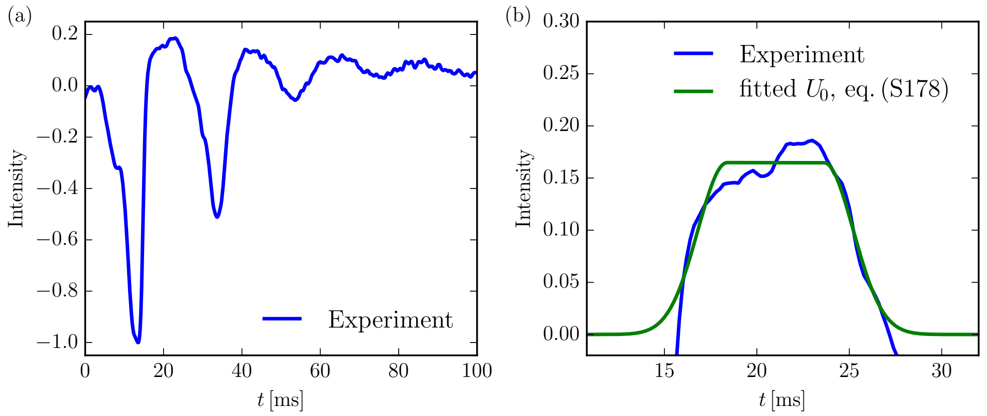


FIG. S12. (a) **Experimentally determined intensity as a function of time**, as recorded by a camera focusing on the razor blade during excitation; (b) **Zoom in on the region around the first positive peak in subplot (a)**, together with fitted function eq. (S178).

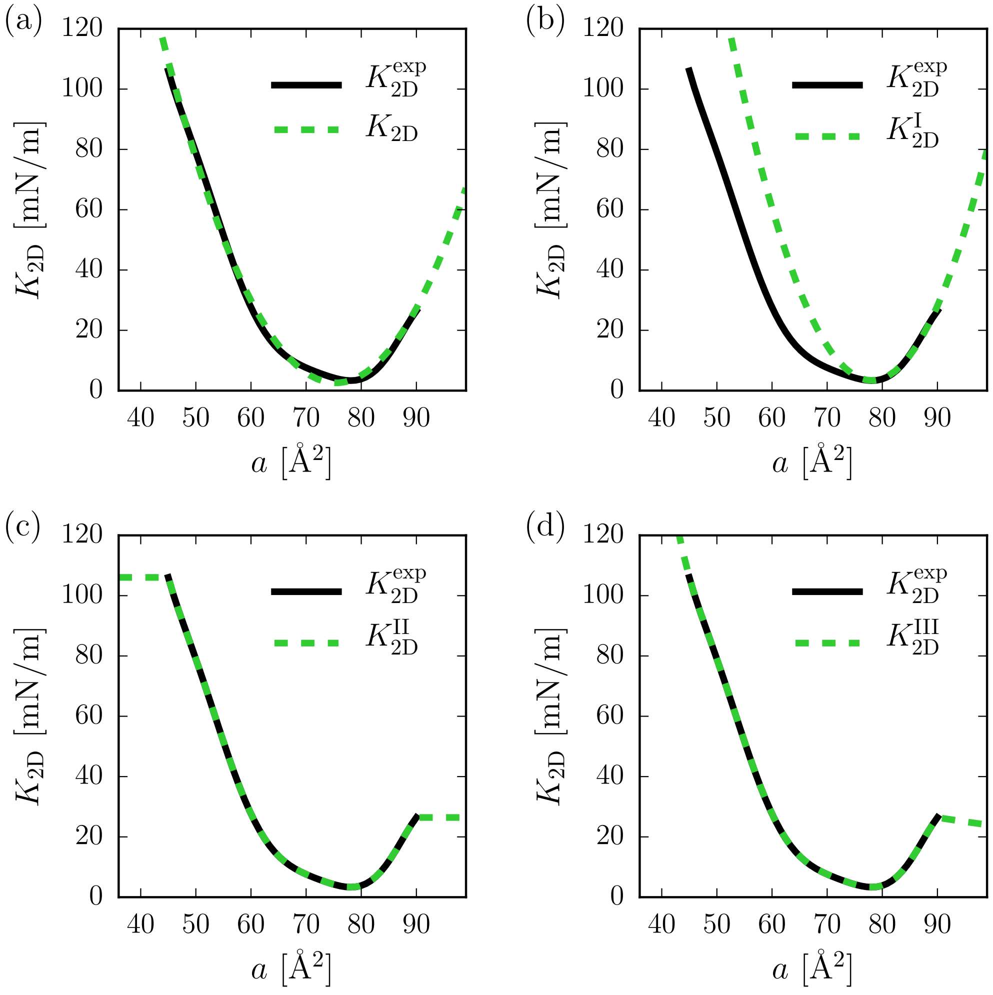


FIG. S13. **Elastic modulus functions considered in sect. S X A.** In all subplots, the black line depicts the experimentally obtained isothermal elastic modulus $K_{2D}^{exp}$ introduced in sect. S III. **(a)** $K_{2D}$**:** The quadratic elastic modulus used in the main text, obtained from fitting a quadratic polynomial to $K_{2D}^{exp}$. **(b)** $K_{2D}^{I}$**:** A quadratic polynomial, fitted to the right of the minimum of $K_{2D}^{exp}$ at around $a_{min} \approx 80\,\text{Å}^2$, with the additional constraint that $K_{2D}^{exp}(a_{min}) = K_{2D}^{I}(a_{min})$. **(c)** $K_{2D}^{II}$**:** The elastic modulus $K_{2D}^{exp}$, extended as constant for $a < 45\,\text{Å}^2$ and $a > 90\,\text{Å}^2$. **(d)** $K_{2D}^{III}$**:** The elastic modulus $K_{2D}^{exp}$ from sect. S III, extrapolated by a second order polynomial for $a < 45\,\text{Å}^2$, and a second oder polynomial in $a^{-1}$ without constant term for $a > 90\,\text{Å}^2$, c.f. eq. (S180). The extensions are chosen such that $K_{2D}^{III}$ and its first derivative are continuous.

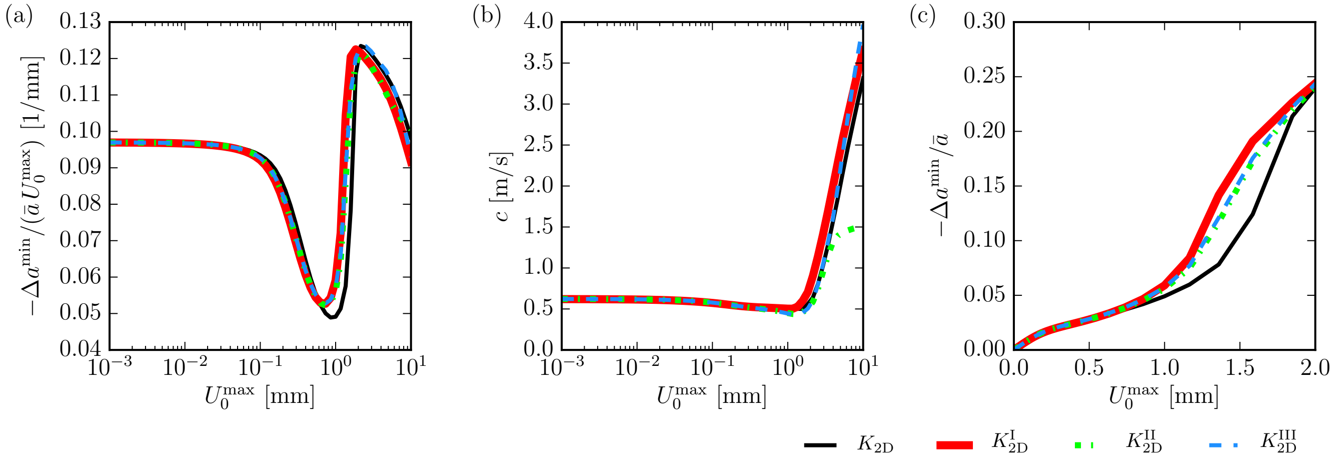


FIG. S14. **Numerical results for area moduli considered in sect. S X A.** Numerical solutions of eq. (17) from the main text with $\rho_{2D} = 0$, with the boundary condition used in the main text, are calculated for the four elastic moduli $K_{2D}$, $K_{2D}^{I}$, $K_{2D}^{II}$, $K_{2D}^{III}$ introduced in sect. S X A and plotted in fig. S13. Calculations are carried out for $\bar{a} = 88.4\,\text{Å}^2$. Using eqs. (28-30) from the main text, maximal compression $-\Delta a^{\min}/\bar{a}$ and wave velocity $c$ are calculated at $x = 8.4$ mm and shown in subplots (a-c) as function of the driving amplitude $U_0^{\max}$.

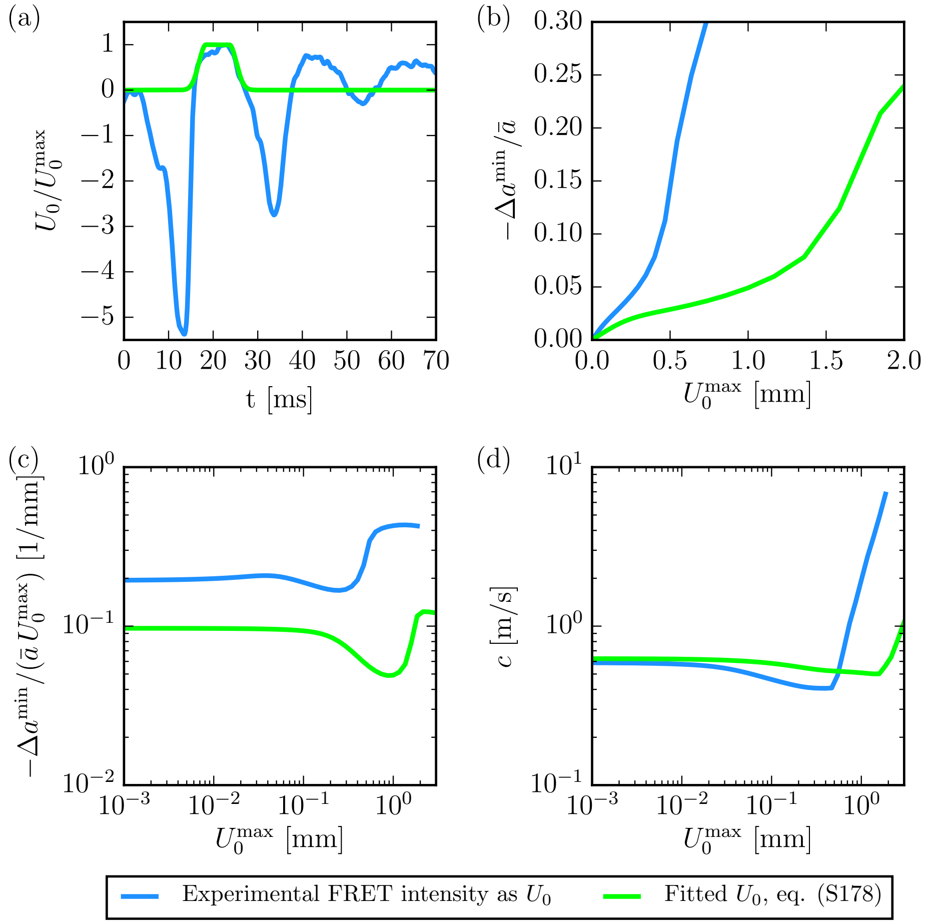


FIG. S15. **Numerical results for recorded intensity profile as boundary condition, as discussed in sect. S X B. Subplot (a)** shows the recorded intensity profile together with the fit from sect. S IX; **Subplot (b)** shows the corresponding maximal compression $-\Delta a^{\min}/\bar{a}$ at a distance $x = 8.4$ mm, as a function of driving amplitude $U_0^{\max}$. As elastic modulus, the quadratic polynomial from the main text is used with $\bar{a} = 88.4\,\text{Å}^2$. **Subplots (c), (d)** show the corresponding relative maximal compression $(-\Delta a^{\min}/\bar{a})/U_0^{\max}$ and the wave speed $c$, c.f. eqs. (28-30) from the main text.

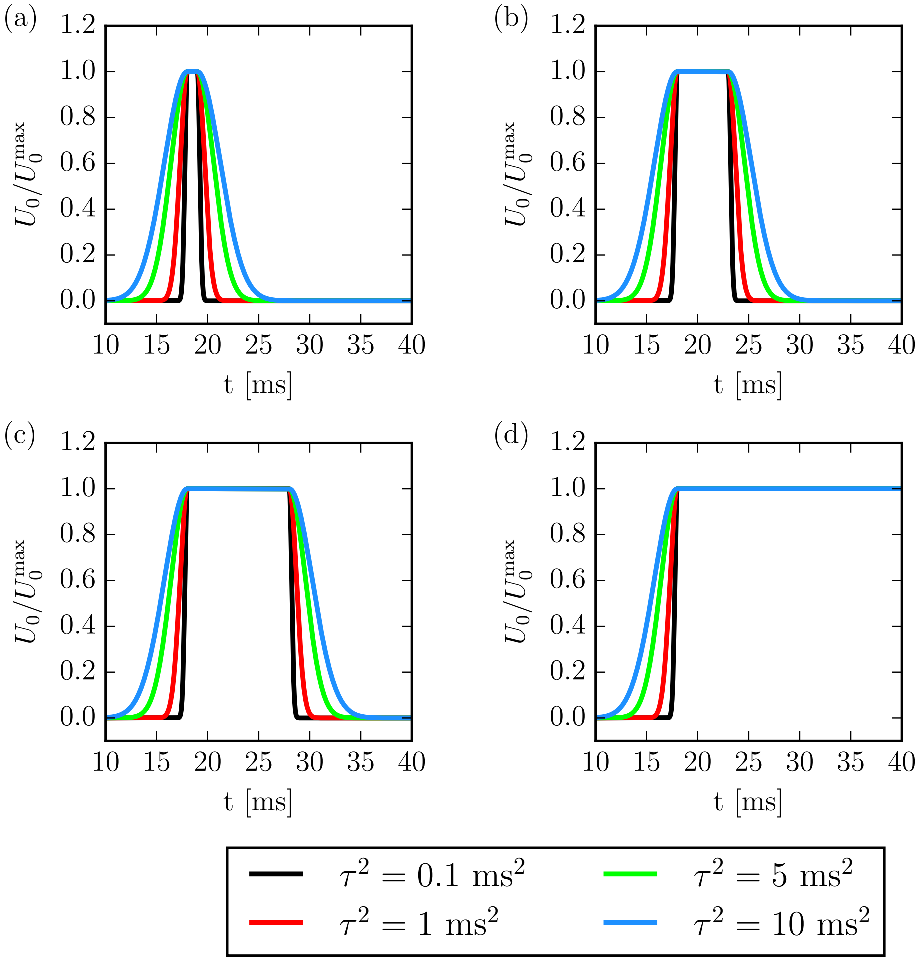


FIG. S16. **Different boundary conditions considered in sect. S X.** All boundary conditions shown here are given by eq. (S181), the corresponding parameters can be found in table I. Plateau widths $\tau_p := t_2 - t_1$ are: **(a)** $\tau_p = 1$ ms; **(b)** $\tau_p = 5$ ms; **(c)** $\tau_p = 10$ ms; **(d)** $\tau_p = \infty$. The results from numerical solutions of the nonlinear fractional wave equation, eq. (23) from the main text, with these boundary conditions are shown in fig. S17.

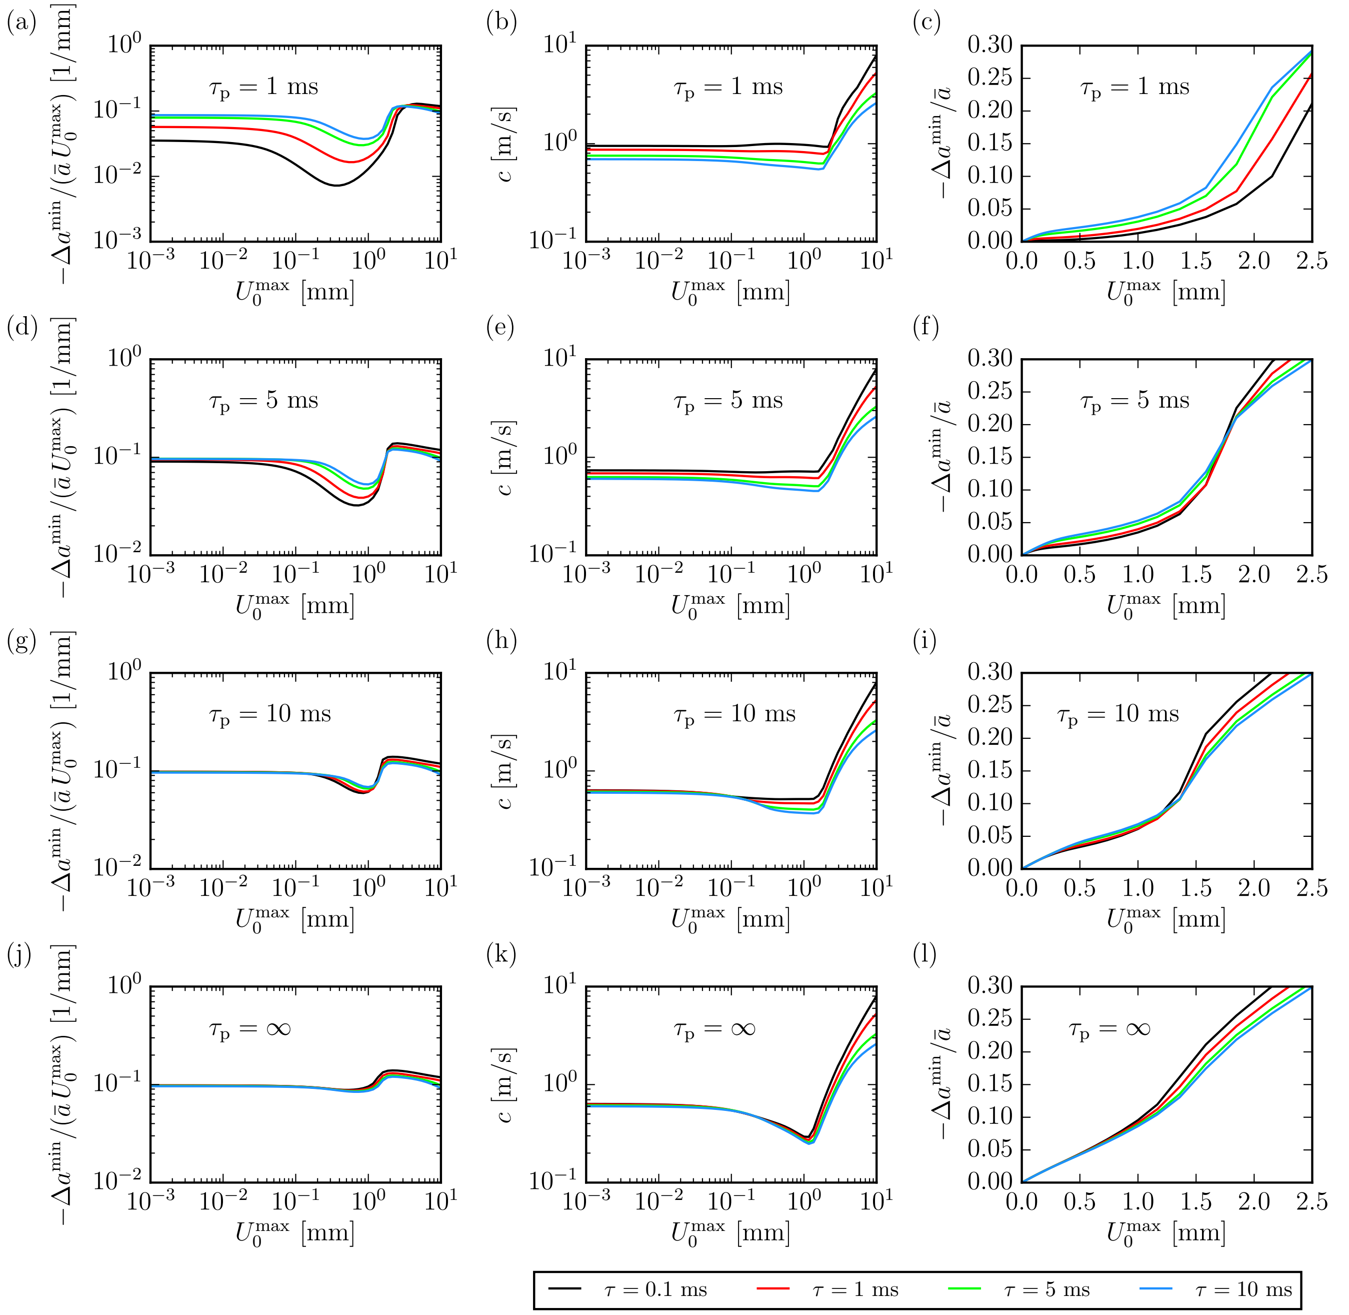


FIG. S17. **Numerical results for different boundary conditions considered in sect. S X.** Equation (23) from the main text is evaluated for each of the boundary conditions shown in fig. S16, with elastic modulus $K_{2\mathrm{D}}$ the quadratic polynomial from the main text at $\bar{a} = 88.4\,\text{Å}^2$. From each solution, maximal compression $-\Delta a^{\mathrm{min}}/\bar{a}$ and wave speed $c$ at $x = 8.4$ mm away from the excitation source are obtained using eqs. (28-30) from the main text. The first row (**subplots (a-c)**) shows the results for the boundary conditions shown in fig. S16 (a). The second row (**subplots (d-f)**) shows the results for the boundary conditions shown in fig. S16 (b). The third row (**subplots (g-i)**) shows the results for the boundary conditions shown in fig. S16 (c). The fourth row (**subplots (j-l)**) shows the results for the boundary conditions shown in fig. S16 (d).
